# Supplementary material for: FoundHand: Large-Scale Domain-Specific Learning for Controllable Hand Image Generation
Source: arXiv:2412.02690 source file (2024-12-04)
Supplement: Supplementary file 1 [file X_suppl.tex]

\clearpage
\setcounter{page}{1}
% \maketitlesupplementary

\makeatletter
  % Store the original section numbering

\setcounter{section}{0}

\section{Gesture Transfer}
In Fig.~\ref{fig:suppl_gesture_transfer}, we showcase results on Gesture Transfer application. 
\modelname generates high quality gesture transferred images and faithfully follows the reference appearance and the target hand pose. In contrast, the baselines which were trained on hands shows limited ability to preserve reference appearance and generates distorted fingers.
Moreover, we try to quantitatively measure the generation ability of our models against baselines in Tab.~\ref{tab:gesture_transfer}.
Therefore, we proposed the identity generation in the main paper, and we show the visual result in Fig.~\ref{fig:suppl_identity}. 
We found that \modelname achieves almost perfect identity generation in all non-cherry picked images, while our baselines~\cite{qin2023unicontrol, sun2024anycontrol, coshand} fails to generate high fidelity results in some times or all times.

\section{Domain Transfer}
In Fig.~\ref{figs:suppl_domain_transfer}, we demonstrate more examples of domain transferred images from ReInterhand~\cite{reinterhand}'s challenging two-hand poses to EpicKitchen~\cite{epickitchen}'s appearances and backgrounds. 
Thanks to strong generalization and appearance preservation of \modelname, our model can be a useful data augmentation tool for dexterity learning.
Specifically, fine-tuned with our domain transferred images, the off-the-shelf hand estimation model~\cite{hamer} shows higher fidelity in very challenging hand images than before fine-tuned.

\section{Novel View Synthesis (NVS)}
We showcase more qualitative examples of novel view synthesis using our model on InterHand2.6M~\cite{interhand} (Fig.~\ref{fig:suppl_nvs} and Fig.~\ref{fig:suppl_nvs2}) and web-sourced in-the-wild images (Fig.~\ref{fig:suppl_nvs_itw}). 
The motivation was that the existing general-purpose methods for novel view synthesis from single images shows very poor quality and fidelity in hands, because of the complex articulation of fingers.
This avoids applications in understanding humans, AR/VR, and human-robot interactions.
Therefore, we repurpose our model to provide realistic novel view synthesis of hands, given only a single image.
Without being explicitly trained on any 3D representations or NVS data, our model can produce remarkably reliable NVS results, even with backgrounds and difficult hand poses.
Notably, compared with baselines~\cite{zeronvs, imagedream} leveraging NeRF~\cite{nerf} to ensure 3D consistency, our geometry-free image generative model demonstrates great 3D understanding of hand.
We found this showing robust 3D piror of hand without explicit 3D geometric context such as depth or mesh template. 

\section{HandFixer}
In Fig.~\ref{fig:suppl_fixhands}, we demonstrate more results in fixing malformed hands.
Generative models could produce malformed hands such as non-five fingers and distorted hand structures. 
% Previously, HandRefiner~\cite{lu2023handrefiner} and RealisHuman~\cite{realishuman} tried to fix this hands, by task-specifically trained on pairs of wrong hands - corrected hands.
% Nevertheless, those methods lack sufficient hand priors and therefore produces less quality results than task-agnostic \modelname.
% Notably, as a versatile model, \modelname, significantly outperforms those methods, without any specific training on fixing hands.
% \modelname can even work with sketches of hands, drawings, challenging hand apperances, and difficult poses interacting with objects.
% It faithfully preserves any handheld objects, backgrounds, and styles of the given malformed hand images, while correctly fixing the hands.
Compared with task-specific methods like HandRefiner~\cite{lu2023handrefiner} and RealisHuman~\cite{realishuman} which requires accurate 3D hand estimation, our \modelname performs zero-shot hand fixing, demonstrating exceptional generalization to diverse artistic and abstract styles. 
\modelname can even work with sketches of hands, drawings, challenging hand apperances, and difficult poses interacting with objects.
The model also shows better understanding of the context, particularly preserving the hand-object interaction context after fixing the hand. 
Moreover, \modelname only requires masks where users want to changes and 2D hand keypoints, which is different from ~\cite{lu2023handrefiner, realishuman} who asks 3D hand models.
This enables more flexible and easier controls for the users to fix hands.

\section{Hand Video and Hand-Object Interaction}
% Given only the first frame and the target 2D hand keypoints in sequence, \modelname can generate a video of hands, despite
% not explicitly trained on videos.
% We provide hand video synthesis results in more details in Fig.~\ref{fig:suppl_video}, where ControlNeXt~\cite{controlnext} often shows artifacts and AnimateAnyone~\cite{animate_anyone} provides limited finger motion. 
% Although ~\cite{controlnext, animate_anyone} models, that we used, were trained on human data and their architectures were specifically designed for video generation only, our results still outperforms those models.
% We conclude that this shows our model’s high versatility and potentials for being used in various applications. 
Given the first frame image and a sequence of 2D keypoints captured in the wild by an iphone camera, \modelname can autoregressively generate a motion-controlled video, despite not explicitly trained on videos. 
This shows our model's high versatility and potentials for being used in various applications. 
We provide hand video synthesis results in more details in Fig.~\ref{fig:suppl_video}, where ControlNeXt~\cite{controlnext} and AnimateAnyone~\cite{animate_anyone} struggles to follow the pose change or present significant visual artifacts, while our model demonstrate robust generalization and emergent understanding of some physical effects such as casted shadows.

Fig.~\ref{fig:suppl_hoi} compares our models' ability to generate hand-object interaction (HOI) videos again the state-of-the-art HOI video synthesis model. 
Note that this involves object translation and deformable objects.
\modelname has naturally seen many hand-object interaction and manipulation scenes and surprisingly develops emergent physical understanding of HOI (object translation and deformation.) without explicit knowledge of the object context. 
On the other hand, CosHand~\cite{coshand} is trained on a set of specific data consisting of before-after pairs of HOI focusing on interaction-induced change.
However, it shows some overfitting such as random objects which we guess were from their training distribution.
% CosHand~\cite{coshand} was directly trained on a small set of before-after pairs of HOI, while ours was not trained on any objects held by hands.
% Nevertheless, \modelname outperforms ~\cite{coshand} significantly, where ~\cite{coshand} occasionally shows some random objects which we guess were from their training distribution.
% On the other hand, as a versatile model, ours shows surprising zero-shot ability towards HOI applications and inherent understanding of hands and their surrounding worlds.

\textbf{Please see supplementary video for video results.}

% Gesture Transfer

\begin{figure*}[!tp]

    \centering \footnotesize
    \begin{tabular}{cccccc}
        \includegraphics[width=0.16\textwidth]{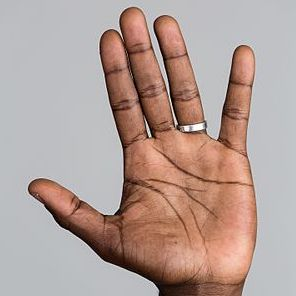}&
        \includegraphics[width=0.16\textwidth]{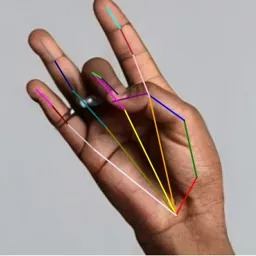}&
        \includegraphics[width=0.16\textwidth]{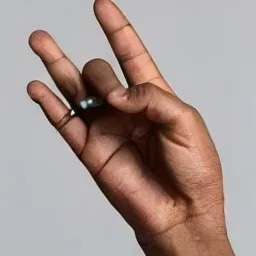}&
        \includegraphics[width=0.16\textwidth]{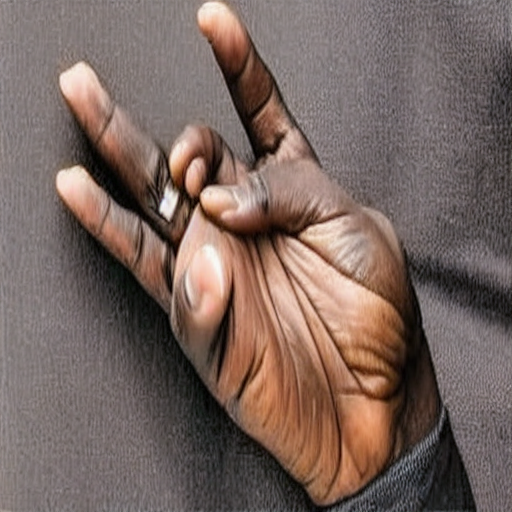} &
        \includegraphics[width=0.16\textwidth]{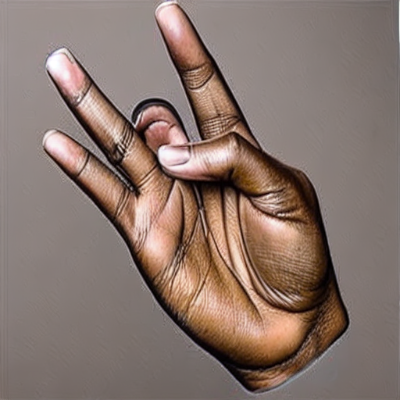}&
        \includegraphics[width=0.16\textwidth]{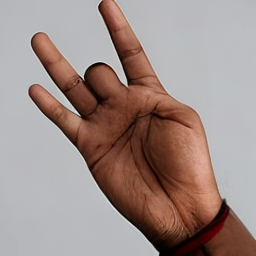} \\
        \includegraphics[width=0.16\textwidth]{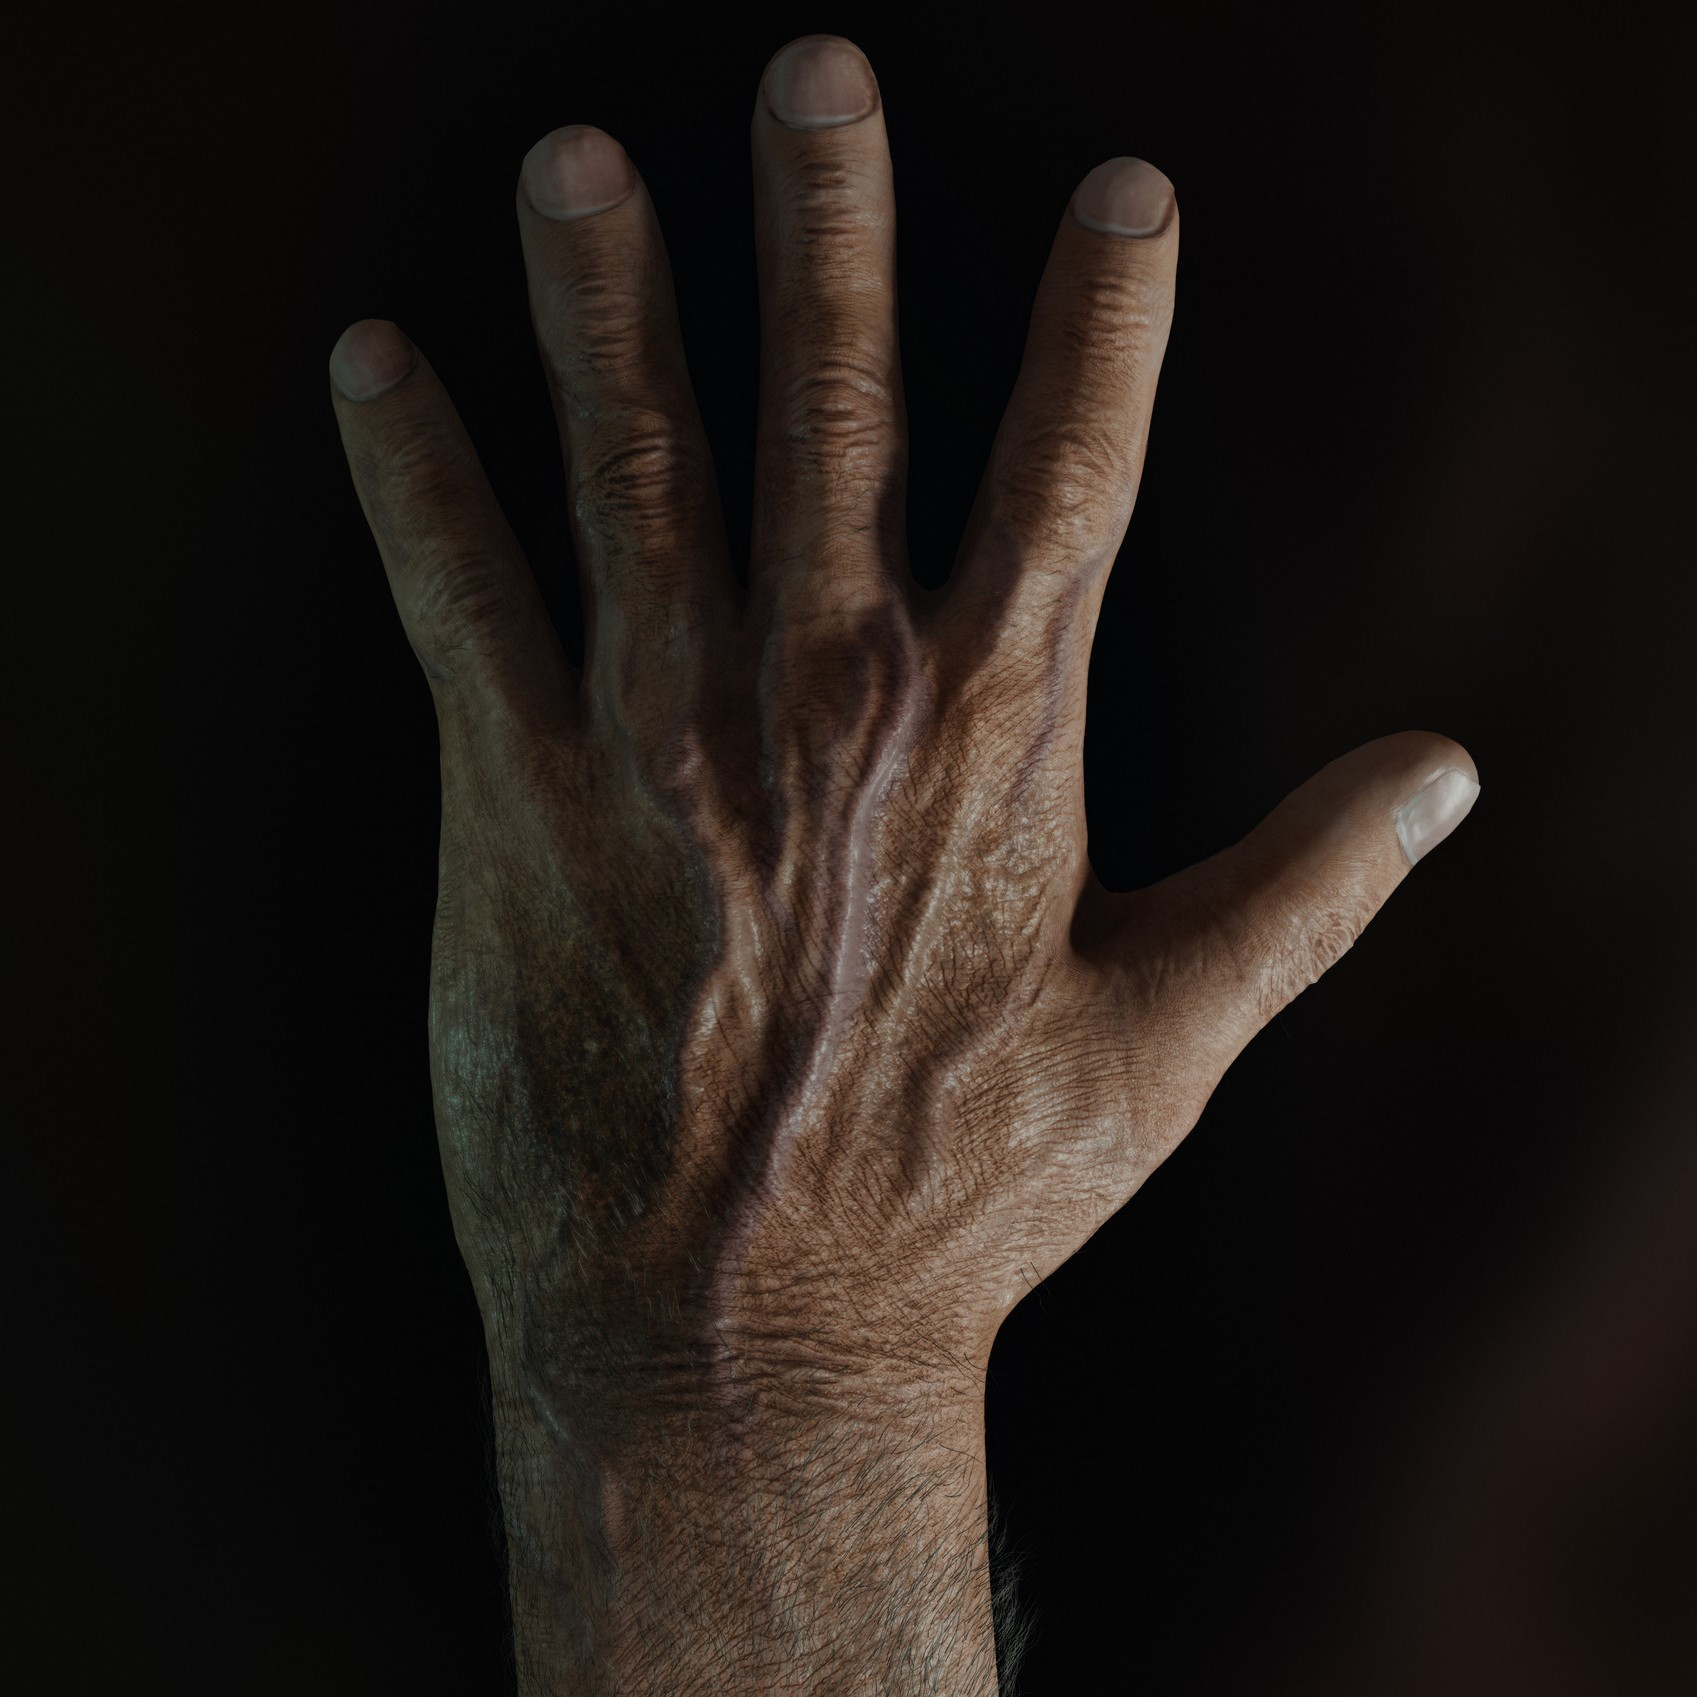}&
        \includegraphics[width=0.16\textwidth]{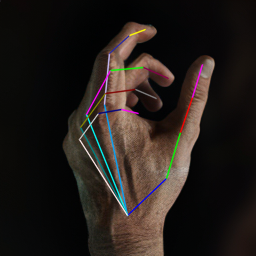}&
        \includegraphics[width=0.16\textwidth]{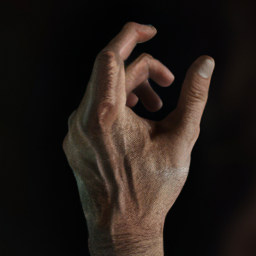}&
        \includegraphics[width=0.16\textwidth]{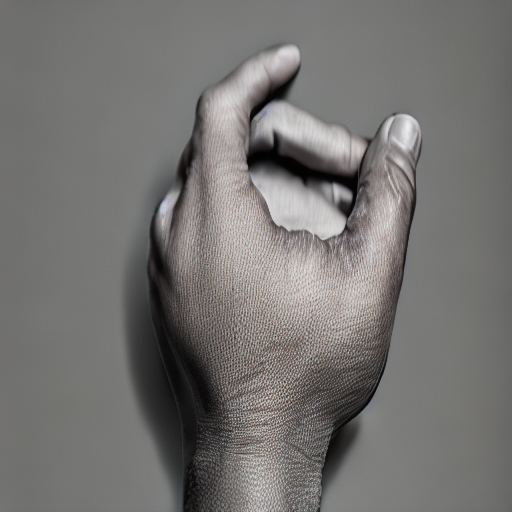} &
        \includegraphics[width=0.16\textwidth]{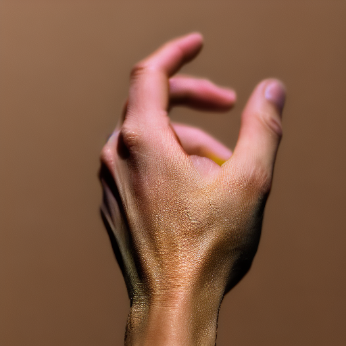} & 
        \includegraphics[width=0.16\textwidth]{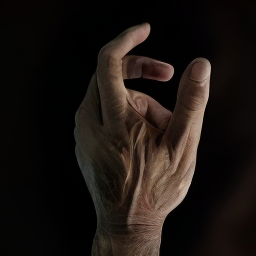}\\
        \includegraphics[width=0.16\textwidth]{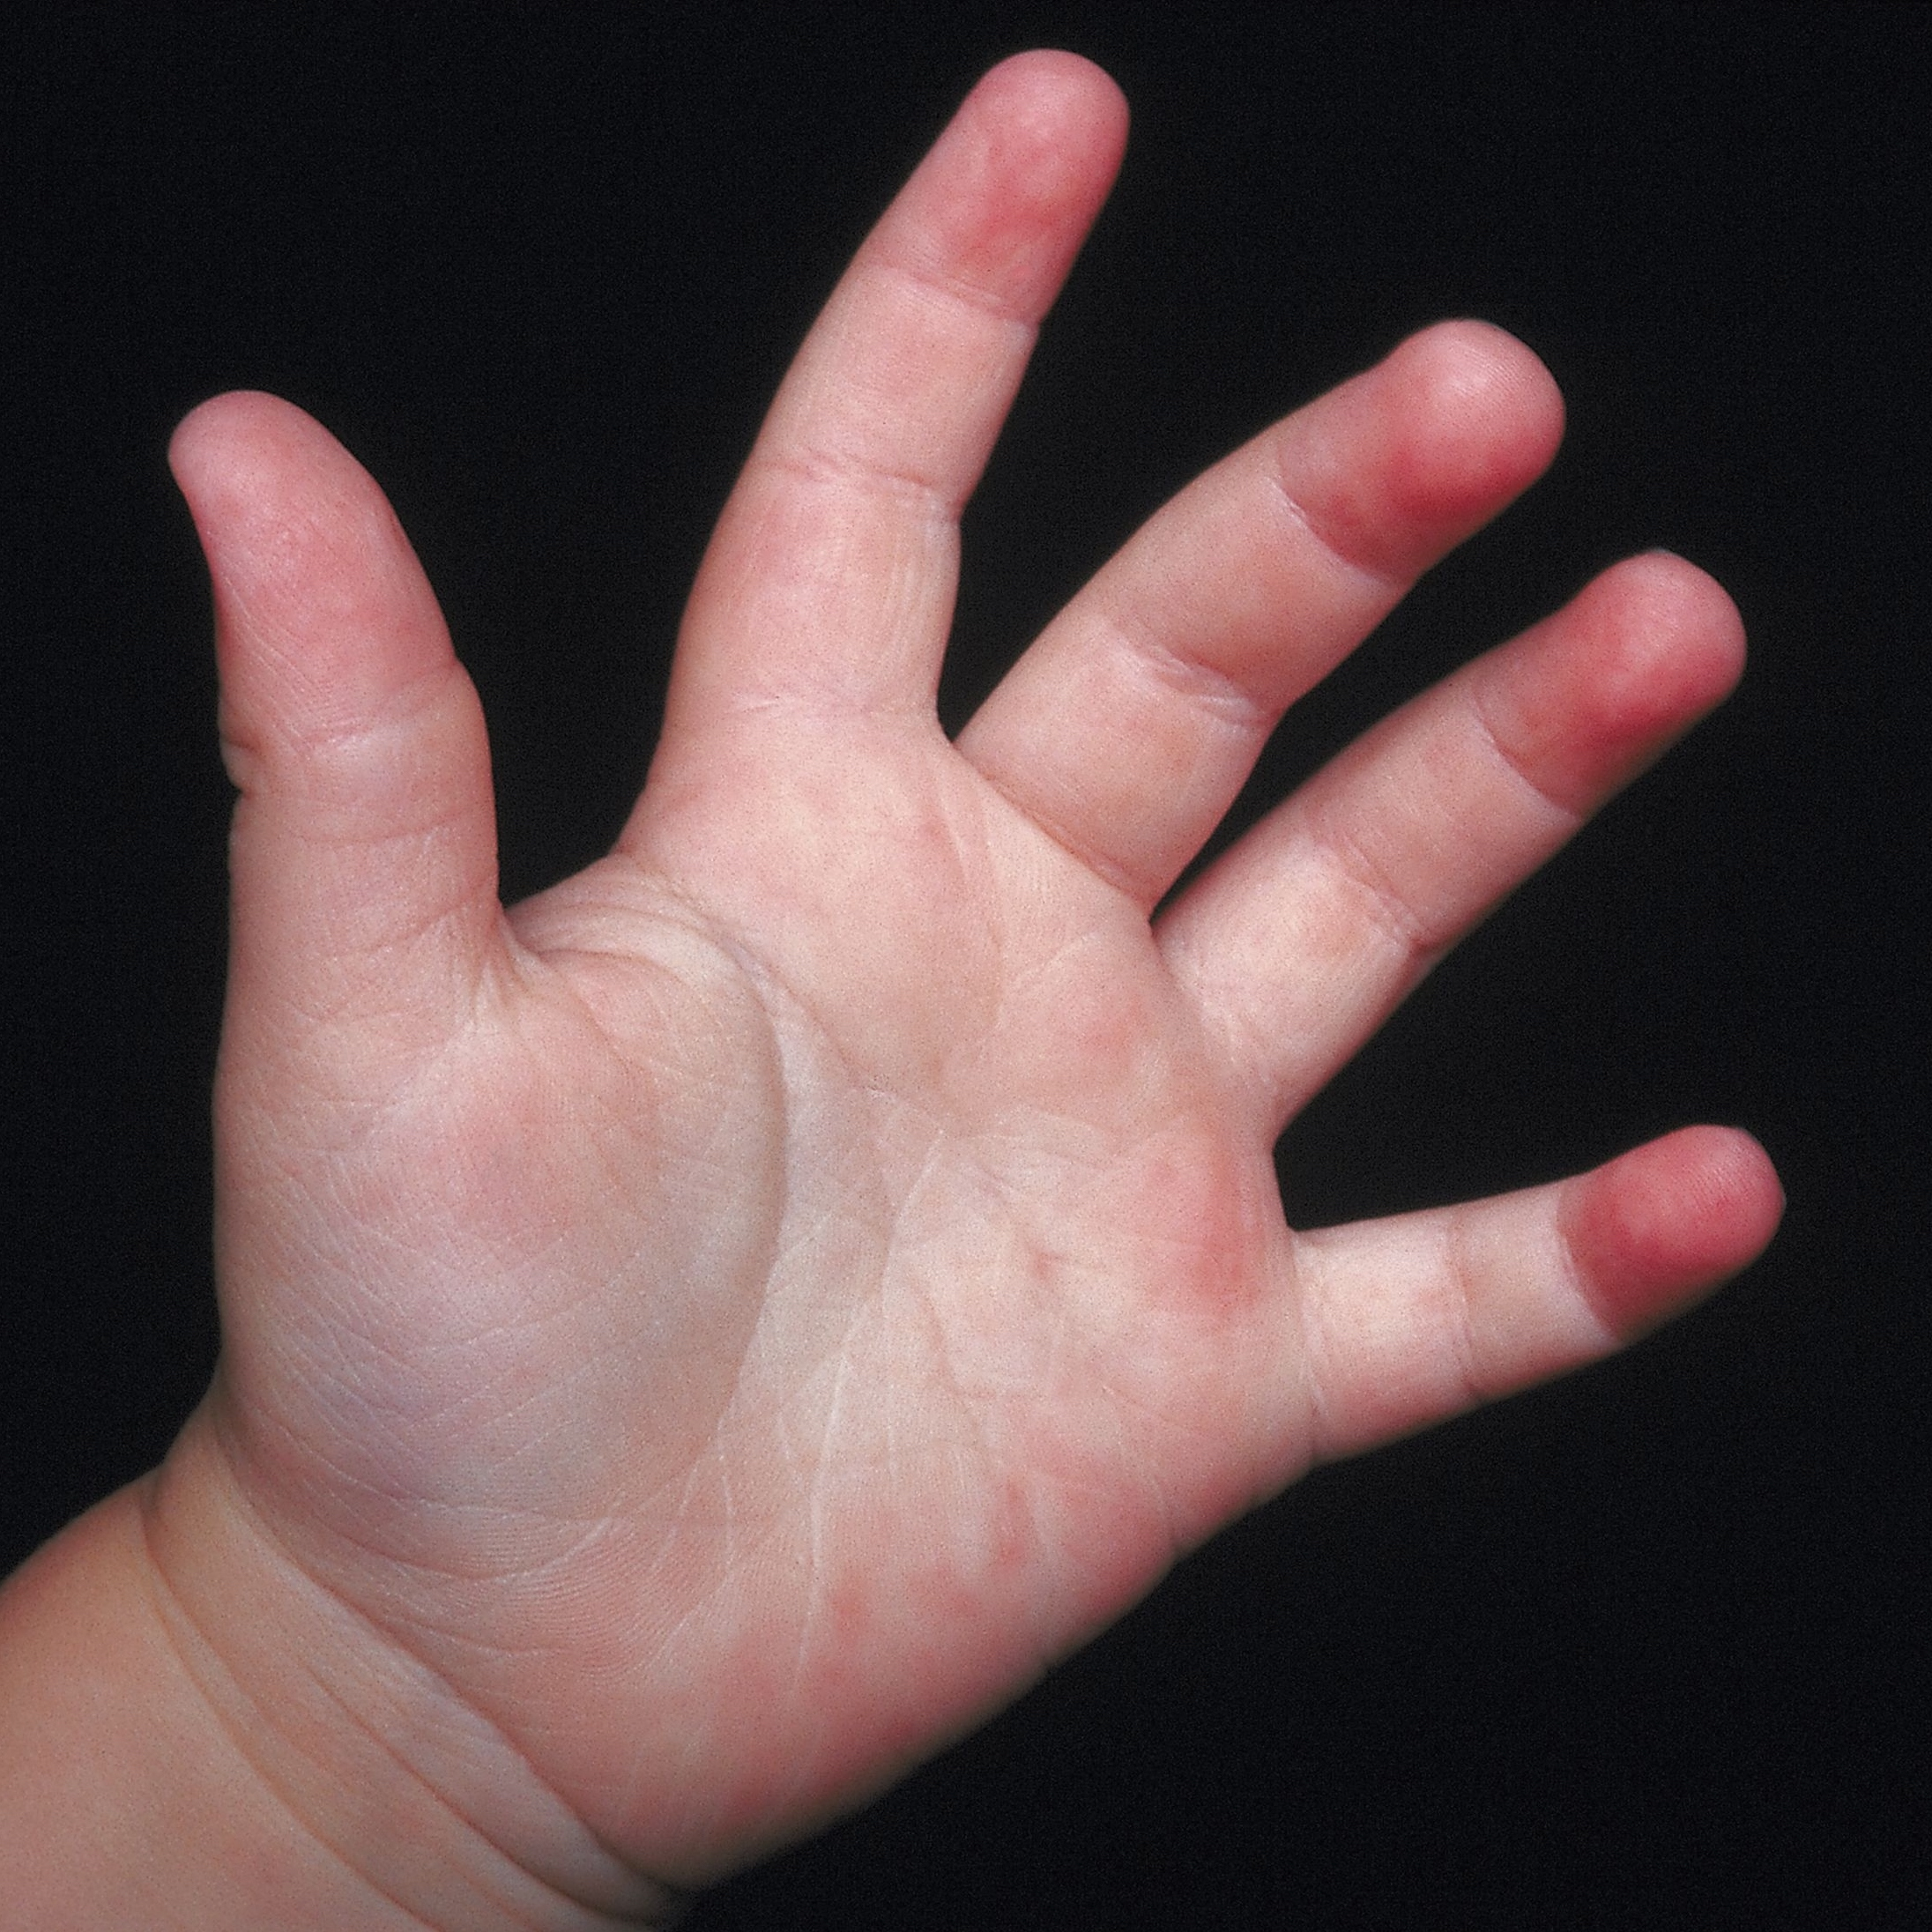}&
        \includegraphics[width=0.16\textwidth]{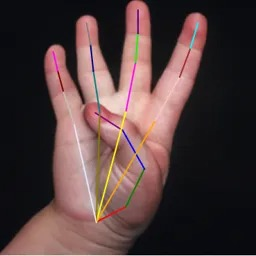}&
        \includegraphics[width=0.16\textwidth]{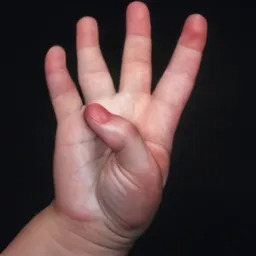}&
        \includegraphics[width=0.16\textwidth]{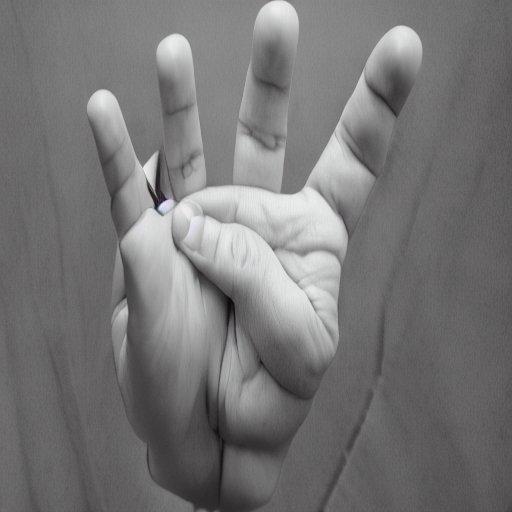} &
        \includegraphics[width=0.16\textwidth]{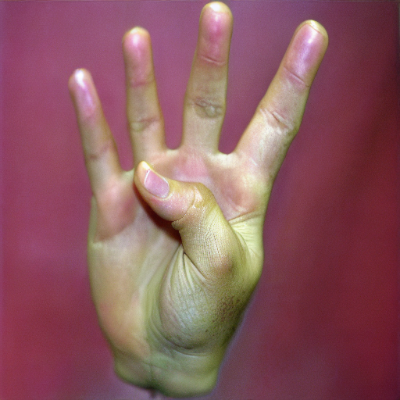} & 
        \includegraphics[width=0.16\textwidth]{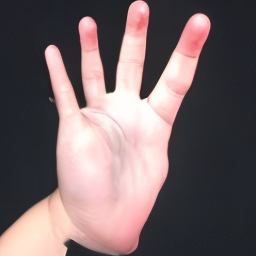}\\
        \includegraphics[width=0.16\textwidth,height=0.16\textwidth]{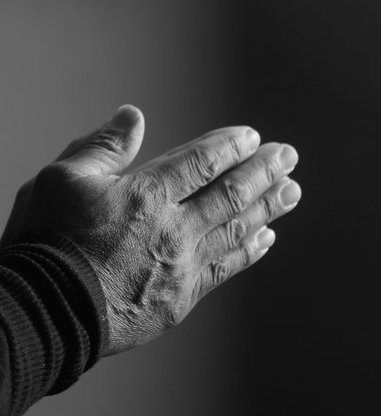}&
        \includegraphics[width=0.16\textwidth]{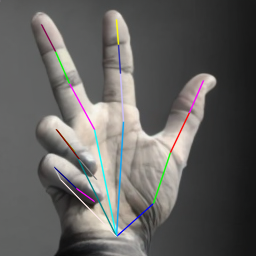}&
        \includegraphics[width=0.16\textwidth]{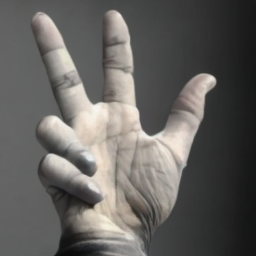}&
        \includegraphics[width=0.16\textwidth]{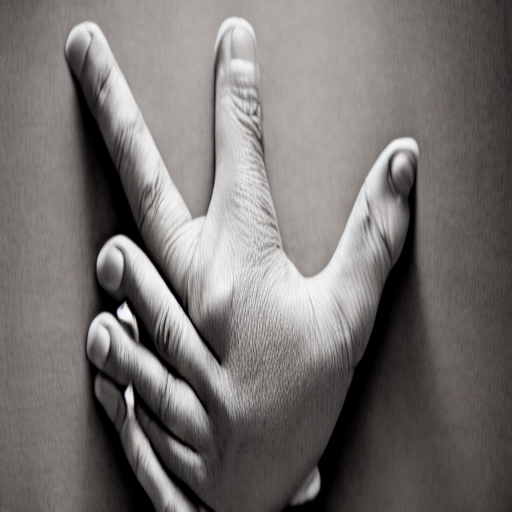} &
        \includegraphics[width=0.16\textwidth]{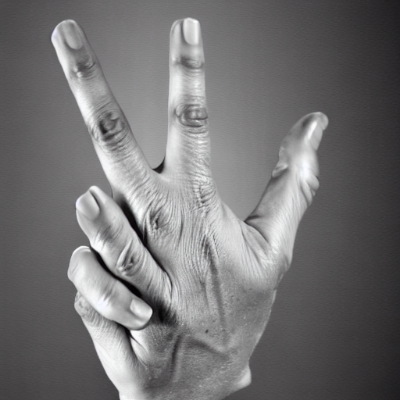} & 
        \includegraphics[width=0.16\textwidth]{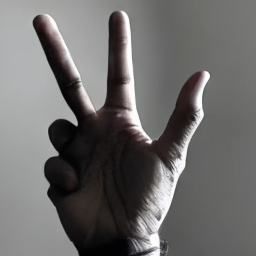}\\
        \includegraphics[width=0.16\textwidth]{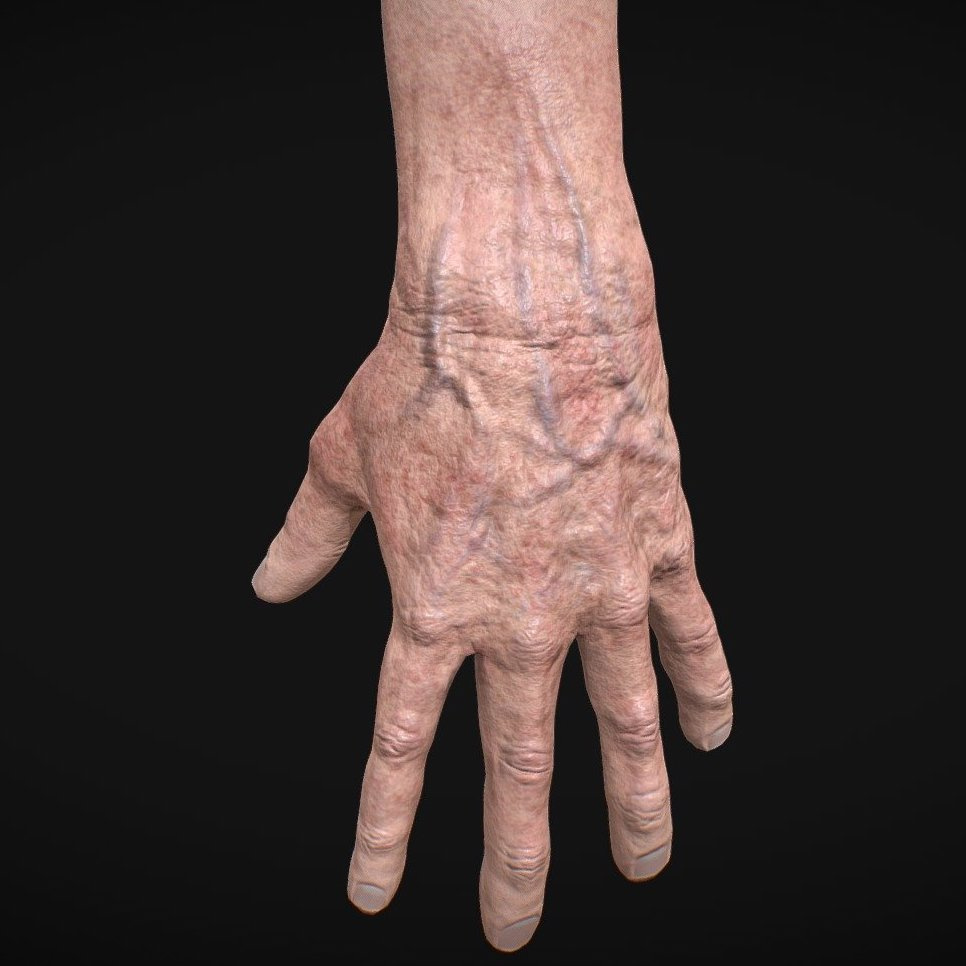}&
        \includegraphics[width=0.16\textwidth]{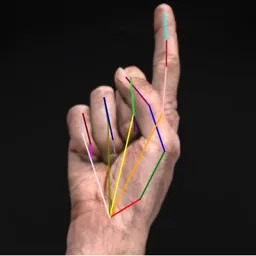}&
        \includegraphics[width=0.16\textwidth]{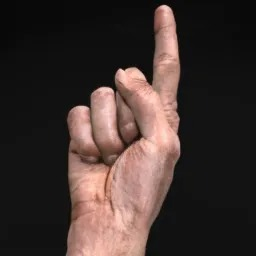}&
        \includegraphics[width=0.16\textwidth]{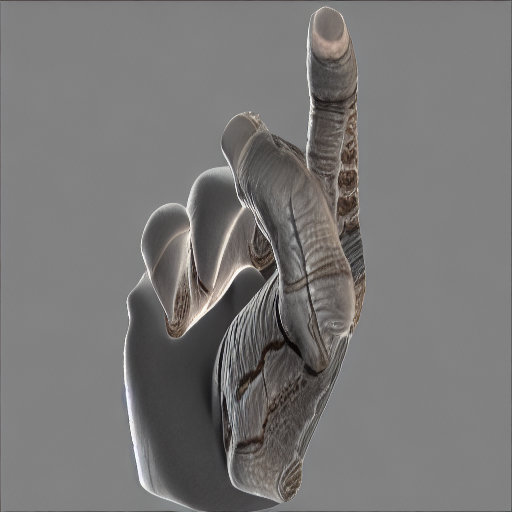} &
        \includegraphics[width=0.16\textwidth]{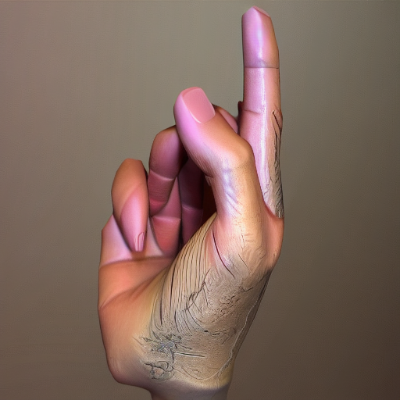} & 
        \includegraphics[width=0.16\textwidth]{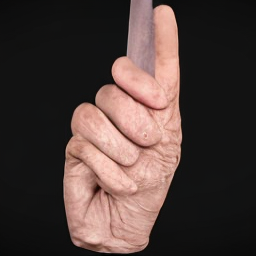}\\
        \includegraphics[width=0.16\textwidth]{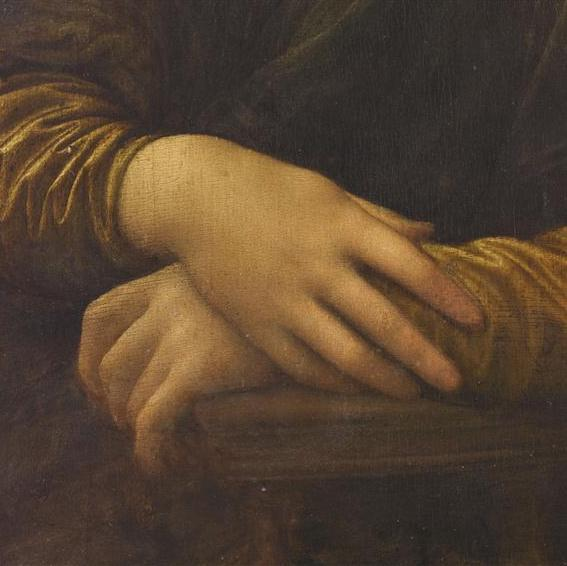}&
        \includegraphics[width=0.16\textwidth]{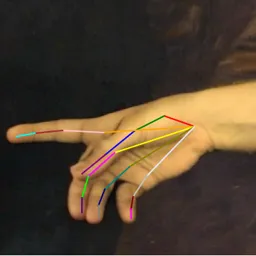}&
        \includegraphics[width=0.16\textwidth]{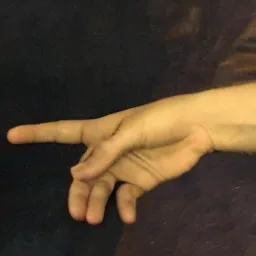}&
        \includegraphics[width=0.16\textwidth]{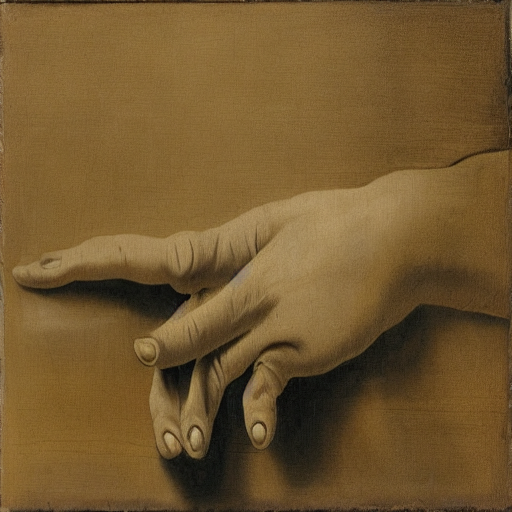} &
        \includegraphics[width=0.16\textwidth]{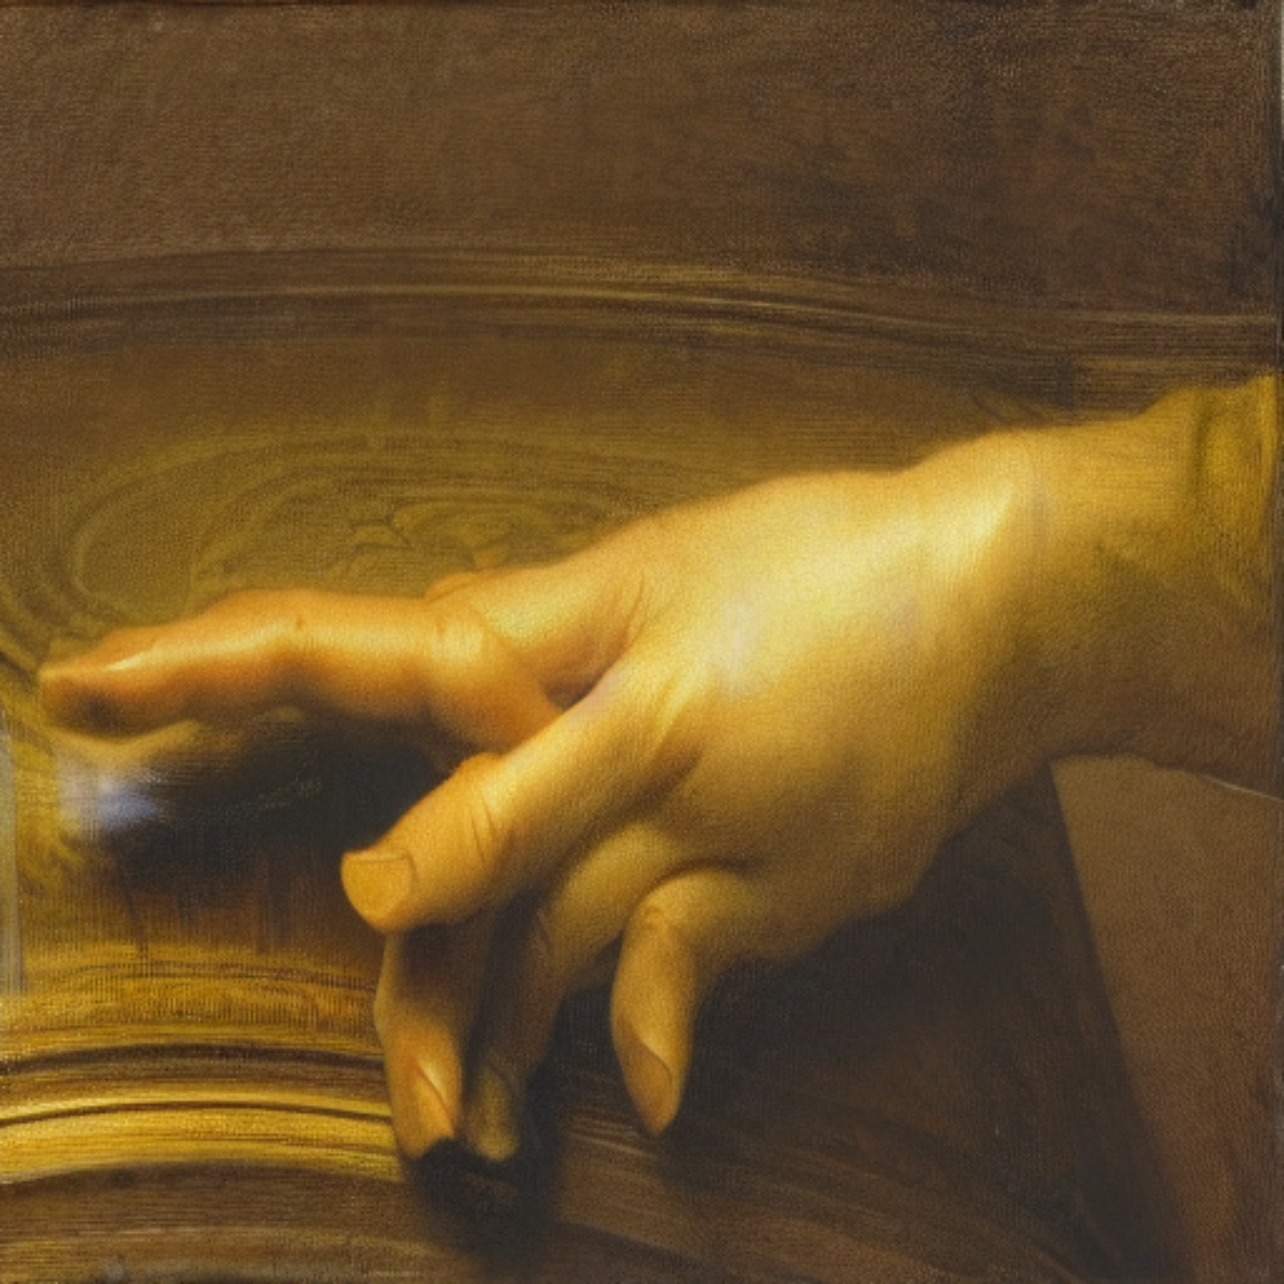} & 
        \includegraphics[width=0.16\textwidth]{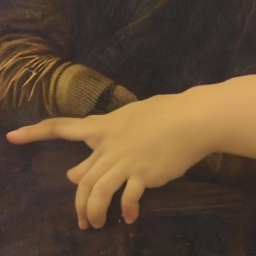}\\
        \includegraphics[width=0.16\textwidth]{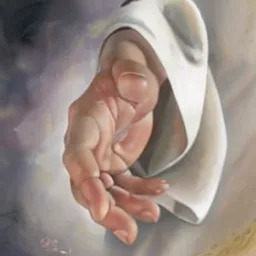}&
        \includegraphics[width=0.16\textwidth]{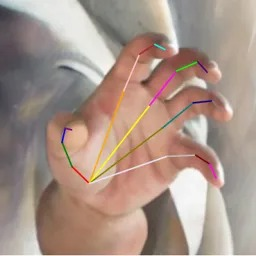}&
        \includegraphics[width=0.16\textwidth]{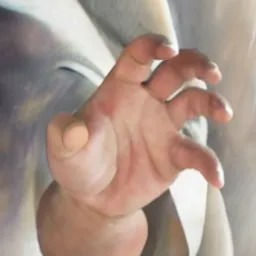}&
        \includegraphics[width=0.16\textwidth,height=0.16\textwidth]{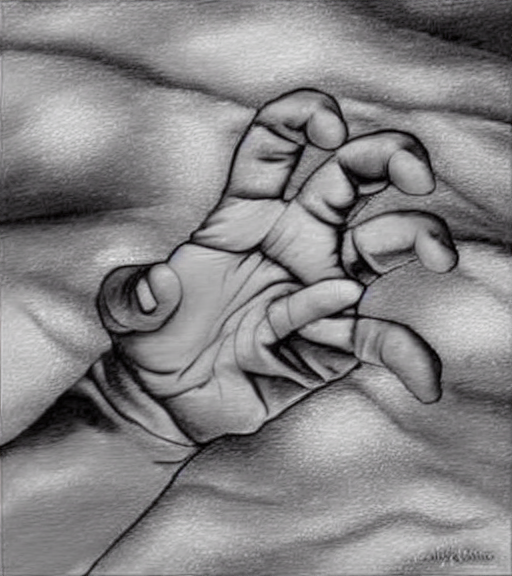} &
        \includegraphics[width=0.16\textwidth,height=0.16\textwidth]{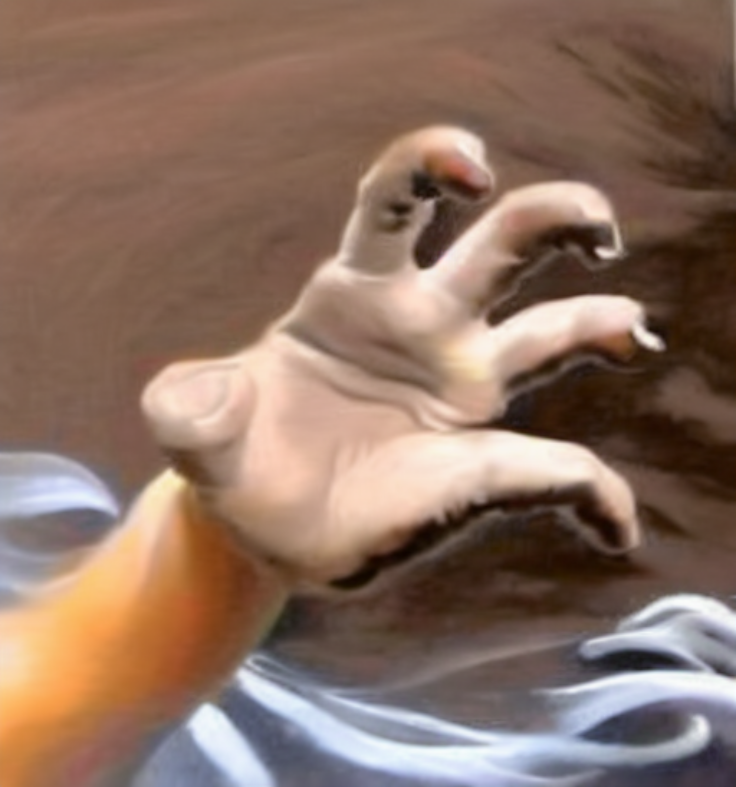} & 
        \includegraphics[width=0.16\textwidth]{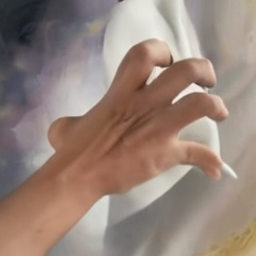}\\ [2.0pt]
        Reference & Ours w/ skeleton & Ours & Uni-ControlNet~\cite{qin2023unicontrol} & AnyControl~\cite{sun2024anycontrol} & CosHand~\cite{coshand}\\
    \end{tabular}
    \caption{More results on Gesture Transfer application. \modelname generates high quality gesture transferred images and faithfully follows the reference appearance and the target hand pose. In contrast, the baselines which were trained on hands shows limited ability to preserve reference appearance and generates distorted fingers.}
    \label{fig:suppl_gesture_transfer}
    % \vspace{-1.5em}
\end{figure*}

% Identity

\begin{figure*}[!tp]

    \centering \footnotesize
    \begin{tabular}{ccccc}
        \includegraphics[width=0.15\textwidth]{figs/gesture_transfer/inputs/sample1.jpg}&
        \includegraphics[width=0.15\textwidth]{figs/gesture_transfer/identity/ours/sample1_identity.png}&
        \includegraphics[width=0.15\textwidth]{figs/gesture_transfer/identity/unicontrolnet/sample1_depth_identity.png} &
        \includegraphics[width=0.15\textwidth]{figs/gesture_transfer/identity/anycontrol/sample1_depth_identity.png}&
        \includegraphics[width=0.15\textwidth]{figs/gesture_transfer/identity/coshand/sample1_identity.png} \\
        \includegraphics[width=0.15\textwidth]{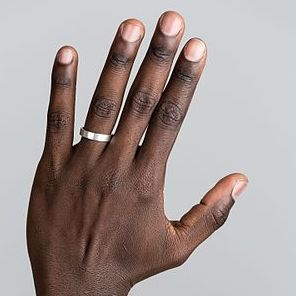}&
        \includegraphics[width=0.15\textwidth]{figs/gesture_transfer/identity/ours/sample2_identity.png}&
        \includegraphics[width=0.15\textwidth]{figs/gesture_transfer/identity/unicontrolnet/sample2_depth_identity.png} &
        \includegraphics[width=0.15\textwidth]{figs/gesture_transfer/identity/anycontrol/sample2_depth_identity.png} & 
        \includegraphics[width=0.15\textwidth]{figs/gesture_transfer/identity/coshand/sample2_identity.png}\\
        \includegraphics[width=0.15\textwidth,height=0.15\textwidth]{figs/gesture_transfer/inputs/sample3.jpg}&
        \includegraphics[width=0.15\textwidth,height=0.15\textwidth]{figs/gesture_transfer/identity/ours/sample3_identity.png}&
        \includegraphics[width=0.15\textwidth,height=0.15\textwidth]{figs/gesture_transfer/identity/unicontrolnet/sample3_depth_identity.png} &
        \includegraphics[width=0.15\textwidth,height=0.15\textwidth]{figs/gesture_transfer/identity/anycontrol/sample3_depth_identity.png} & 
        \includegraphics[width=0.15\textwidth,height=0.15\textwidth]{figs/gesture_transfer/identity/coshand/sample3_identity.png}\\
        \includegraphics[width=0.15\textwidth]{figs/gesture_transfer/inputs/sample4.jpg}&
        \includegraphics[width=0.15\textwidth]{figs/gesture_transfer/identity/ours/sample4_identity.png}&
        \includegraphics[width=0.15\textwidth]{figs/gesture_transfer/identity/unicontrolnet/sample4_depth_identity.png} &
        \includegraphics[width=0.15\textwidth]{figs/gesture_transfer/identity/anycontrol/sample4_depth_identity.png} & 
        \includegraphics[width=0.15\textwidth]{figs/gesture_transfer/identity/coshand/sample4_identity.png}\\
        \includegraphics[width=0.15\textwidth]{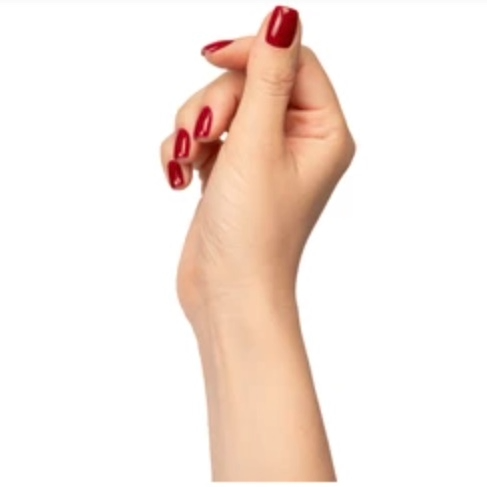}&
        \includegraphics[width=0.15\textwidth]{figs/gesture_transfer/identity/ours/sample6_identity.png}&
        \includegraphics[width=0.15\textwidth]{figs/gesture_transfer/identity/unicontrolnet/sample6_depth_identity.png} &
        \includegraphics[width=0.15\textwidth]{figs/gesture_transfer/identity/anycontrol/sample6_depth_identity.png} & 
        \includegraphics[width=0.15\textwidth]{figs/gesture_transfer/identity/coshand/sample6_identity.png}\\
        \includegraphics[width=0.15\textwidth]{figs/gesture_transfer/inputs/sample8.jpg}&
        \includegraphics[width=0.15\textwidth]{figs/gesture_transfer/identity/ours/sample8_identity.png}&
        \includegraphics[width=0.15\textwidth]{figs/gesture_transfer/identity/unicontrolnet/sample8_depth_identity.png} &
        \includegraphics[width=0.15\textwidth]{figs/gesture_transfer/identity/anycontrol/sample8_depth_identity.png} & 
        \includegraphics[width=0.15\textwidth]{figs/gesture_transfer/identity/coshand/sample8_identity.png}\\
        \includegraphics[width=0.15\textwidth]{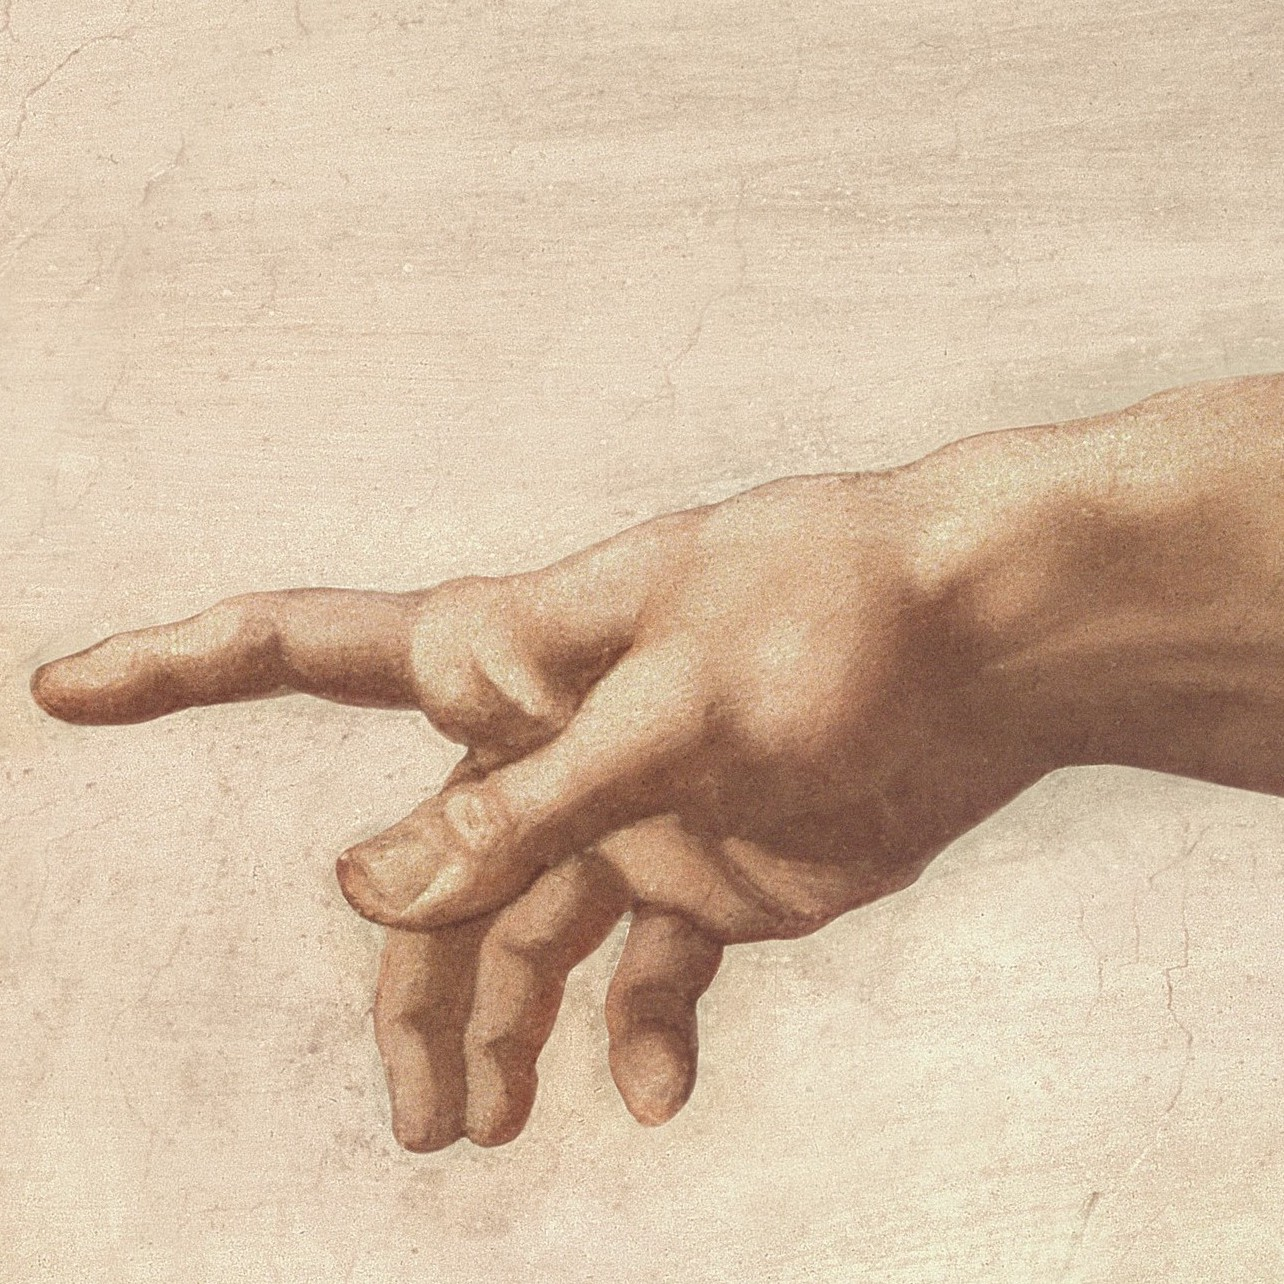}&
        \includegraphics[width=0.15\textwidth]{figs/gesture_transfer/identity/ours/sample10_identity.png}&
        \includegraphics[width=0.15\textwidth]{figs/gesture_transfer/identity/unicontrolnet/sample10_depth_identity.png} &
        \includegraphics[width=0.15\textwidth]{figs/gesture_transfer/identity/anycontrol/sample10_depth_identity.png} & 
        \includegraphics[width=0.15\textwidth]{figs/gesture_transfer/identity/coshand/sample10_identity.png}\\
        \includegraphics[width=0.15\textwidth]{figs/gesture_transfer/inputs/sample11.jpg}&
        \includegraphics[width=0.15\textwidth]{figs/gesture_transfer/identity/ours/sample11_identity.png}&
        \includegraphics[width=0.15\textwidth]{figs/gesture_transfer/identity/unicontrolnet/sample11_depth_identity.png} &
        \includegraphics[width=0.15\textwidth]{figs/gesture_transfer/identity/anycontrol/sample11_depth_identity.png} & 
        \includegraphics[width=0.15\textwidth]{figs/gesture_transfer/identity/coshand/sample11_identity.png}\\
[2.0pt]
        Reference & Ours & Uni-ControlNet~\cite{qin2023unicontrol} & AnyControl~\cite{sun2024anycontrol} & CosHand~\cite{coshand}\\
    \end{tabular}
    \caption{Identity generation to quantitatively measure the generation ability of \modelname and baselines. \modelname achieves almost perfect reconstruction in all examples, while the baselines occasionally or always fail to generate high fidelity results.}
    \label{fig:suppl_identity}
    % \vspace{-1.5em}
\end{figure*}

% Domain Transfer 

\begin{figure*}[!tp]

    \centering \footnotesize
    \begin{tabular}{cccccc}
    \includegraphics[width=0.15\textwidth]{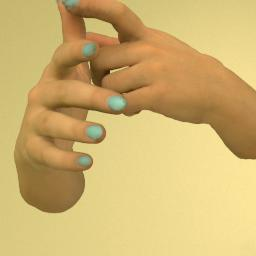} & 
    \includegraphics[width=0.15\textwidth]{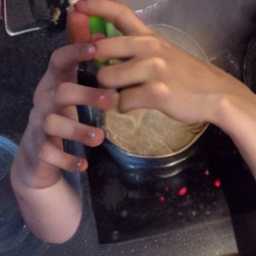} & 
    \includegraphics[width=0.15\textwidth]{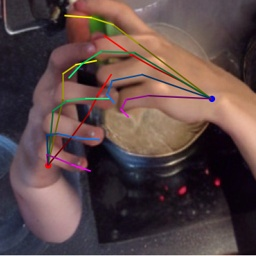} & 
    \includegraphics[width=0.15\textwidth]{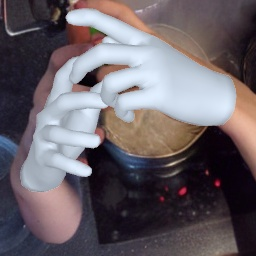} & 
    \includegraphics[width=0.15\textwidth]{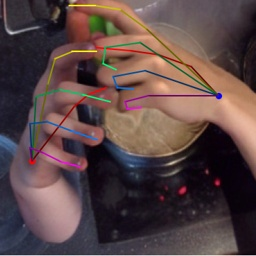} & 
    \includegraphics[width=0.15\textwidth]{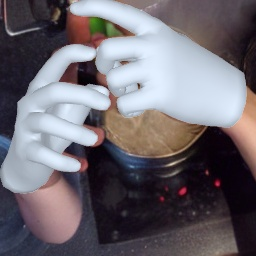} \\ 
    \includegraphics[width=0.15\textwidth]{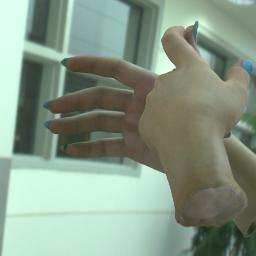} & 
    \includegraphics[width=0.15\textwidth]{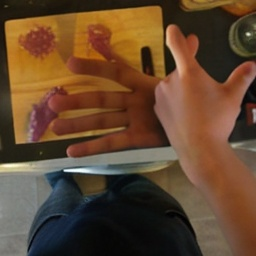} & 
    \includegraphics[width=0.15\textwidth]{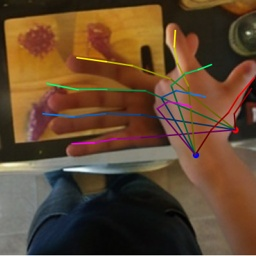} & 
    \includegraphics[width=0.15\textwidth]{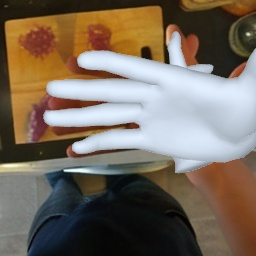} & 
    \includegraphics[width=0.15\textwidth]{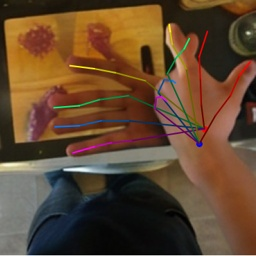} & 
    \includegraphics[width=0.15\textwidth]{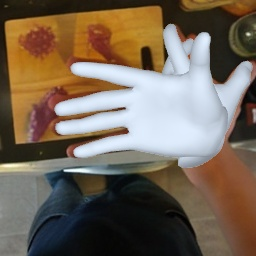} \\ 
    \includegraphics[width=0.15\textwidth]{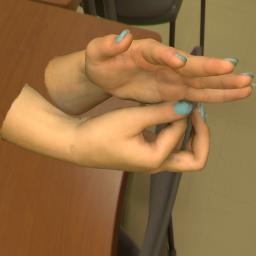} & 
    \includegraphics[width=0.15\textwidth]{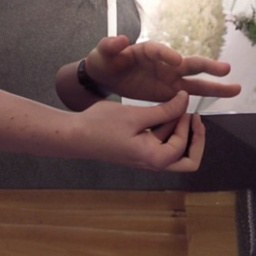} & 
    \includegraphics[width=0.15\textwidth]{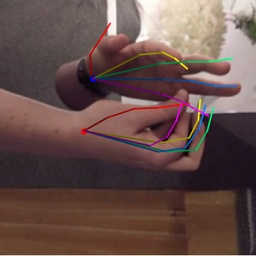} & 
    \includegraphics[width=0.15\textwidth]{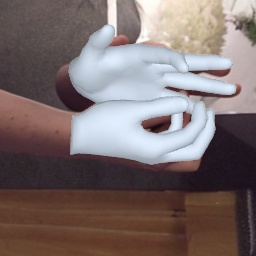} & 
    \includegraphics[width=0.15\textwidth]{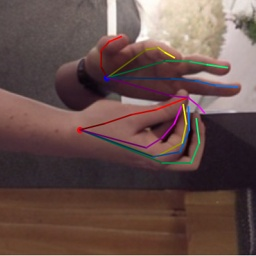} & 
    \includegraphics[width=0.15\textwidth]{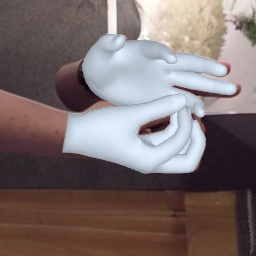} \\ 
    \includegraphics[width=0.15\textwidth]{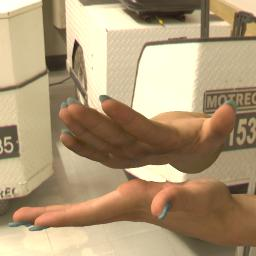} & 
    \includegraphics[width=0.15\textwidth]{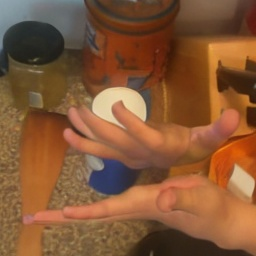} & 
    \includegraphics[width=0.15\textwidth]{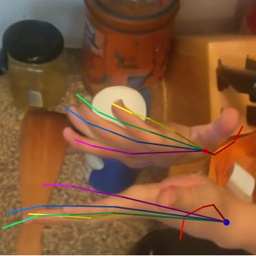} & 
    \includegraphics[width=0.15\textwidth]{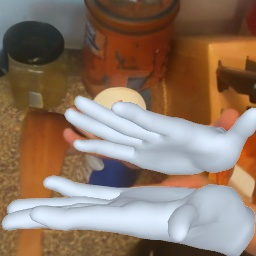} & 
    \includegraphics[width=0.15\textwidth]{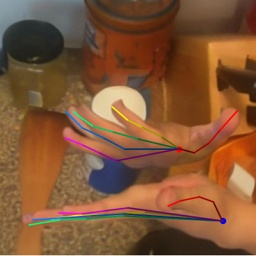} & 
    \includegraphics[width=0.15\textwidth]{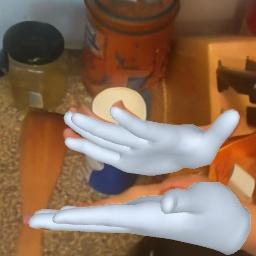} \\ 
    \includegraphics[width=0.15\textwidth]{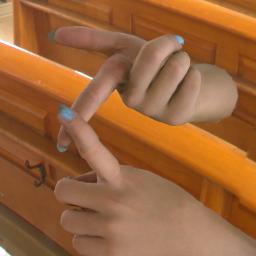} & 
    \includegraphics[width=0.15\textwidth]{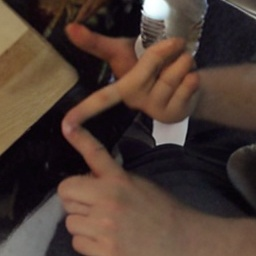} & 
    \includegraphics[width=0.15\textwidth]{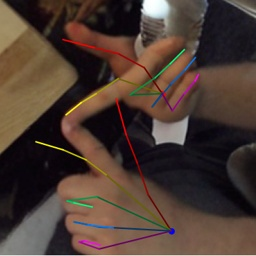} & 
    \includegraphics[width=0.15\textwidth]{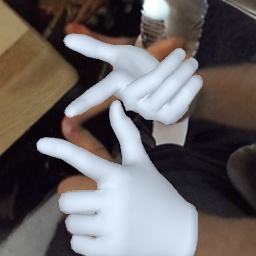} & 
    \includegraphics[width=0.15\textwidth]{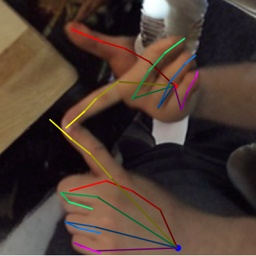} & 
    \includegraphics[width=0.15\textwidth]{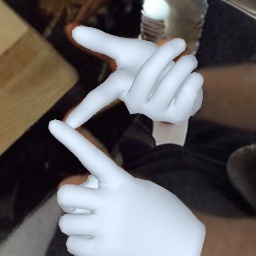} \\ 
    \includegraphics[width=0.15\textwidth]{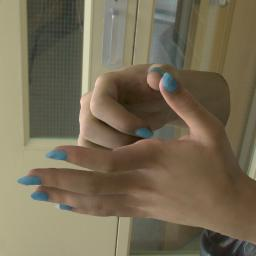} & 
    \includegraphics[width=0.15\textwidth]{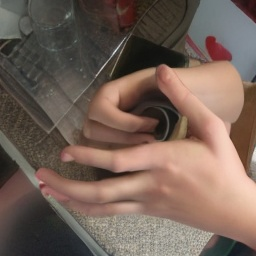} & 
    \includegraphics[width=0.15\textwidth]{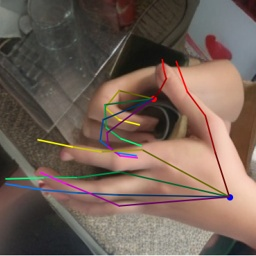} & 
    \includegraphics[width=0.15\textwidth]{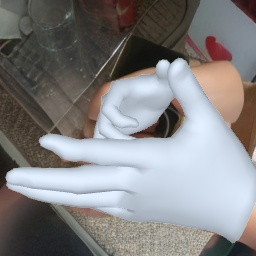} & 
    \includegraphics[width=0.15\textwidth]{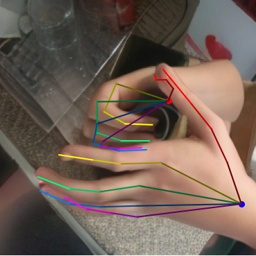} & 
    \includegraphics[width=0.15\textwidth]{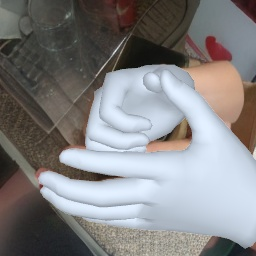} \\ 
    \includegraphics[width=0.15\textwidth]{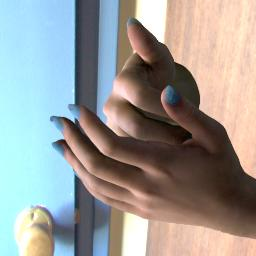} & 
    \includegraphics[width=0.15\textwidth]{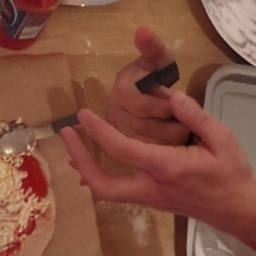} & 
    \includegraphics[width=0.15\textwidth]{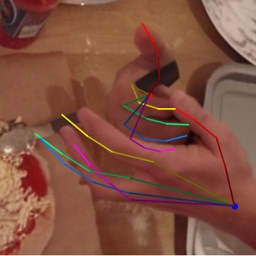} & 
    \includegraphics[width=0.15\textwidth]{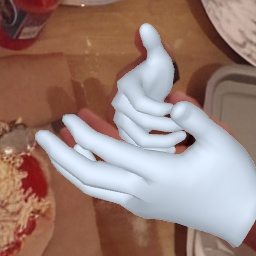} & 
    \includegraphics[width=0.15\textwidth]{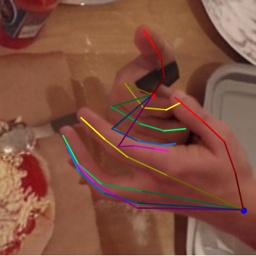} & 
    \includegraphics[width=0.15\textwidth]{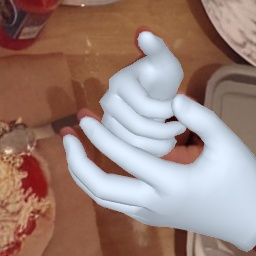} \\ [3.0pt]
    Synthetic data & Domain transferred & \multicolumn{2}{c}{Before finetuning} & \multicolumn{2}{c}{After finetuning}\\
    \end{tabular}
    \caption{\modelname can provide domain transfer from highly complex hand poses from synthetic data~\cite{reinterhand} and reference images from real-world data~\cite{epickitchen}. Fine-tuned with our domain transferred images, the off-the-shelf hand estimation model~\cite{hamer} shows even higher fidelity in very challenging hand images.}
    \label{figs:suppl_domain_transfer}
\end{figure*}

% NVS with comparisons
\begin{figure*}[!tp]

    \centering \footnotesize
    \begin{tabular}{ccccccccc}
    \rotatebox{90}{\hspace{1.1cm} \footnotesize\cite{zeronvs}} & 
    \; &
    \includegraphics[width=0.15\textwidth]{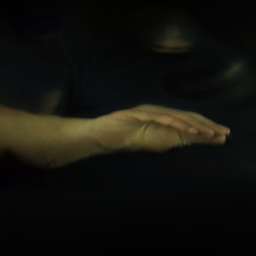} & 
    \includegraphics[width=0.15\textwidth]{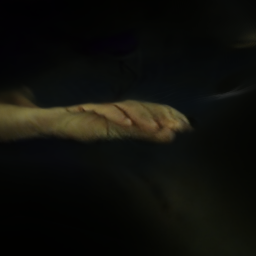} & 
    \includegraphics[width=0.15\textwidth]{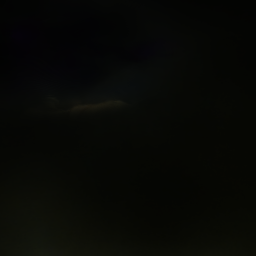} & 
    \includegraphics[width=0.15\textwidth]{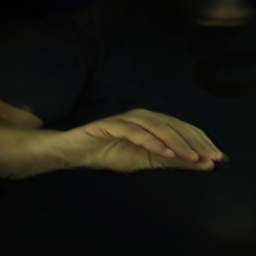} & 
    \includegraphics[width=0.15\textwidth]{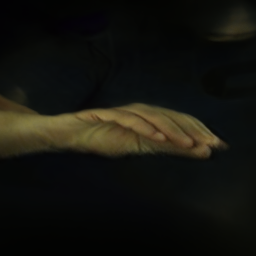} & 
    \includegraphics[width=0.15\textwidth]{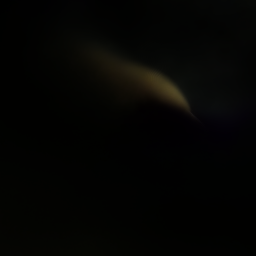} \\
    \rotatebox{90}{\hspace{1.3cm}\footnotesize \cite{imagedream}\;}&
    &
    \includegraphics[width=0.15\textwidth]{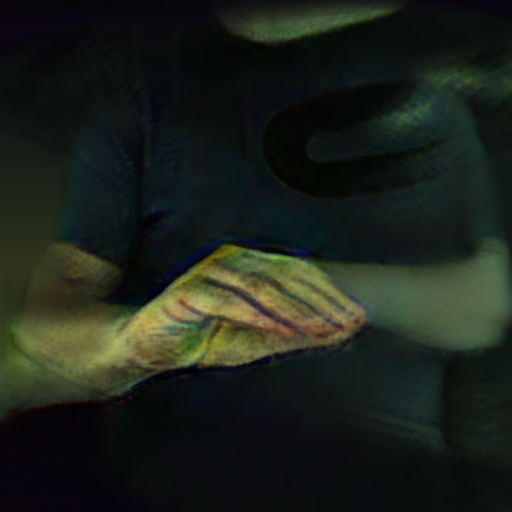} & 
    \includegraphics[width=0.15\textwidth]{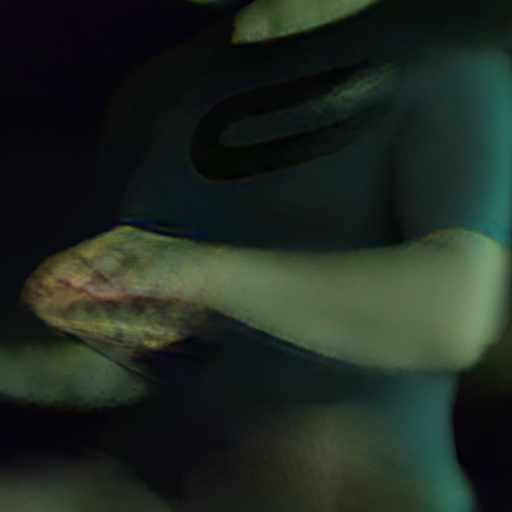} & 
    \includegraphics[width=0.15\textwidth]{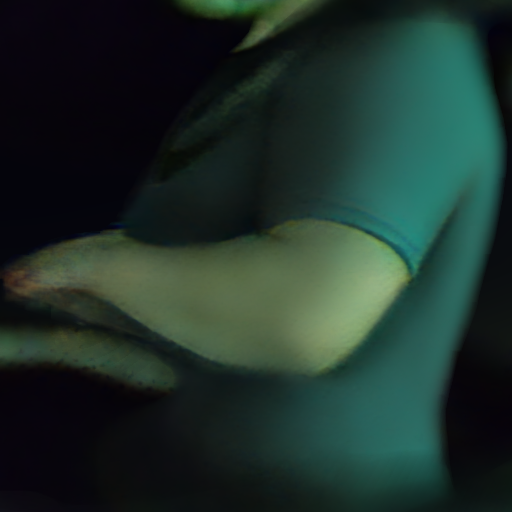} & 
    \includegraphics[width=0.15\textwidth]{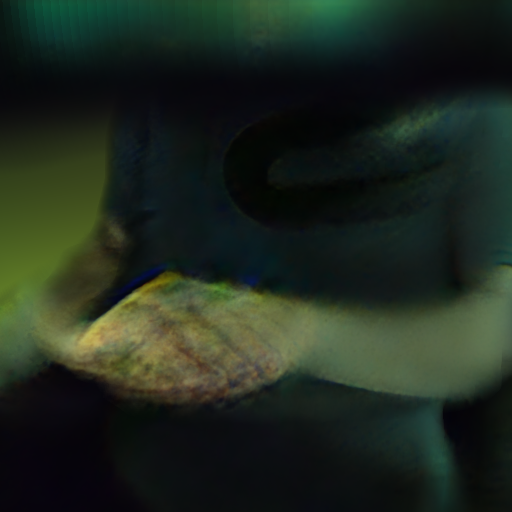} & 
    \includegraphics[width=0.15\textwidth]{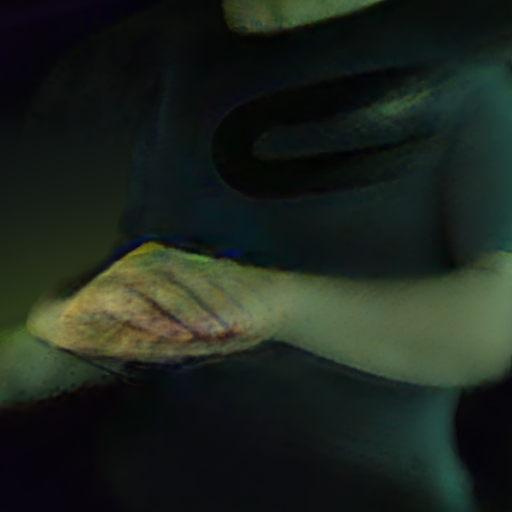} & 
    \includegraphics[width=0.15\textwidth]{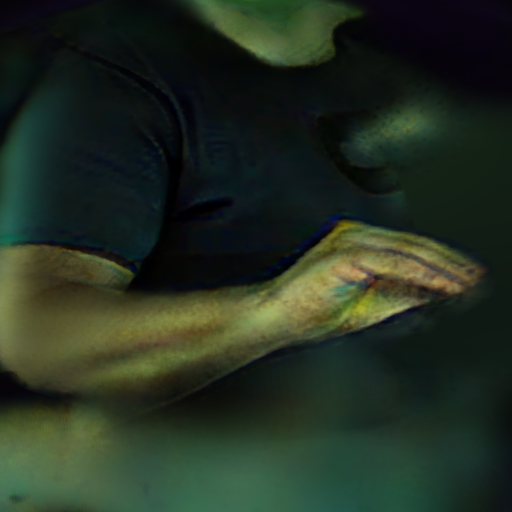} \\
    \rotatebox{90}{\hspace{1.2cm}\footnotesize Ours\;}&
    &
    \includegraphics[width=0.15\textwidth]{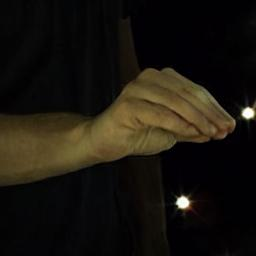} & 
    \includegraphics[width=0.15\textwidth]{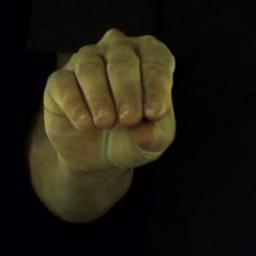} & 
    \includegraphics[width=0.15\textwidth]{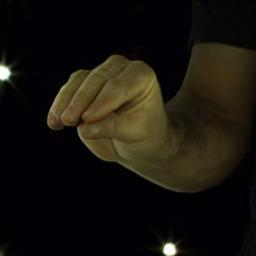} & 
    \includegraphics[width=0.15\textwidth]{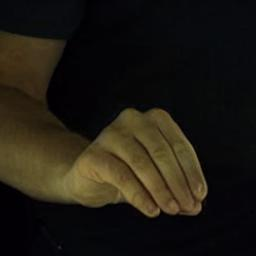} & 
    \includegraphics[width=0.15\textwidth]{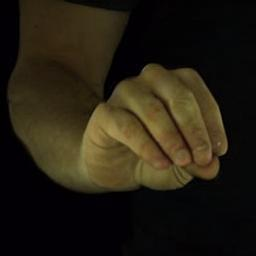} & 
    \includegraphics[width=0.15\textwidth]{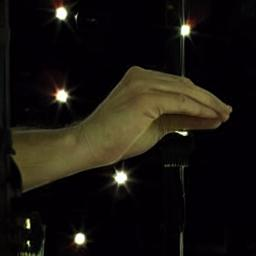} \\
    \rotatebox{90}{\hspace{1.2cm}\footnotesize GT\;}&
    &
    \includegraphics[width=0.15\textwidth]{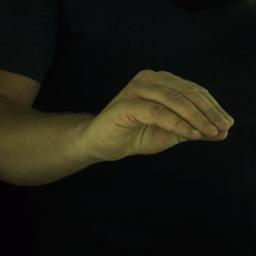} & 
    \includegraphics[width=0.15\textwidth]{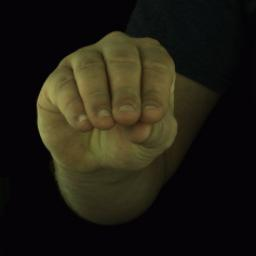} & 
    \includegraphics[width=0.15\textwidth]{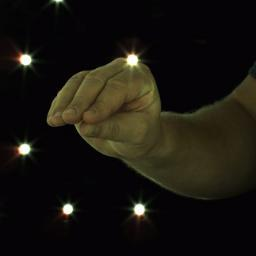} & 
    \includegraphics[width=0.15\textwidth]{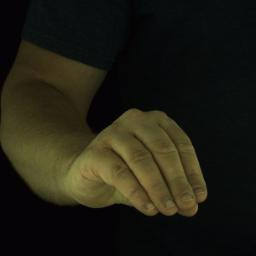} & 
    \includegraphics[width=0.15\textwidth]{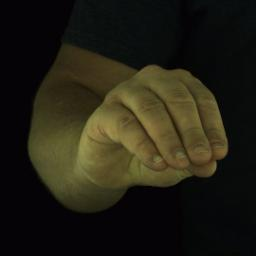} & 
    \includegraphics[width=0.15\textwidth]{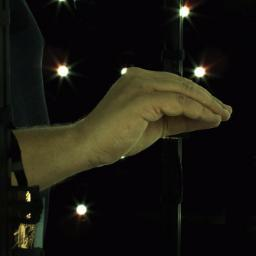} \\[3.0pt]
    \rotatebox{90}{\hspace{1.0cm} \footnotesize\cite{zeronvs}} & 
    \; &
    \includegraphics[width=0.15\textwidth]{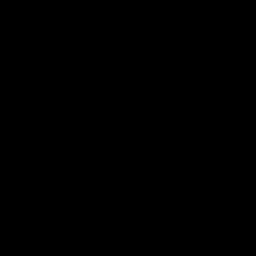} & 
    \includegraphics[width=0.15\textwidth]{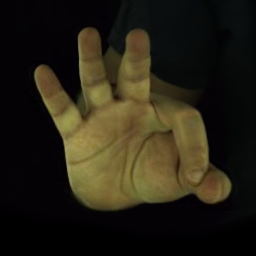} & 
    \includegraphics[width=0.15\textwidth]{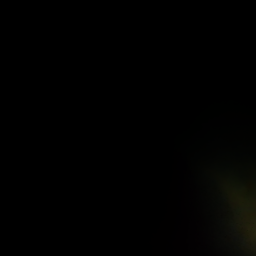} & 
    \includegraphics[width=0.15\textwidth]{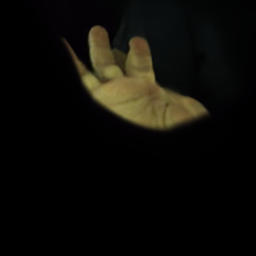} & 
    \includegraphics[width=0.15\textwidth]{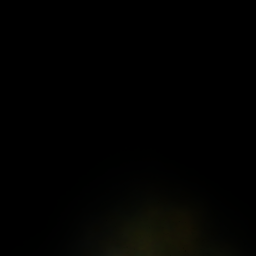} & 
    \includegraphics[width=0.15\textwidth]{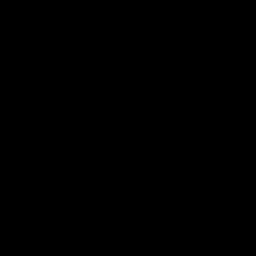} \\
    \rotatebox{90}{\hspace{1.0cm}\footnotesize \cite{imagedream}\;}&
    &
    \includegraphics[width=0.15\textwidth]{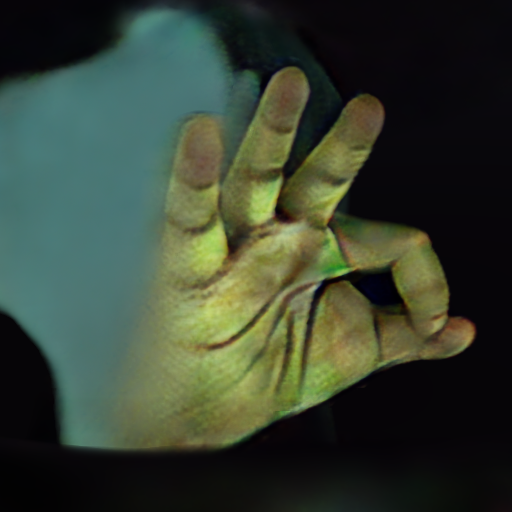} & 
    \includegraphics[width=0.15\textwidth]{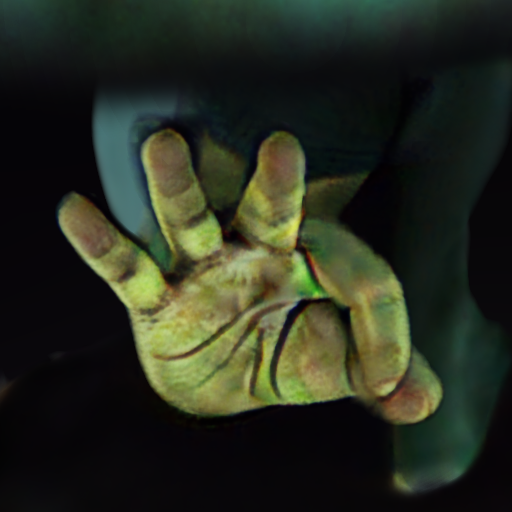} & 
    \includegraphics[width=0.15\textwidth]{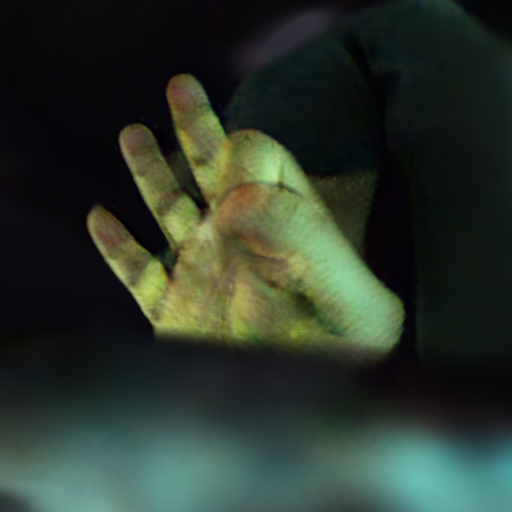} & 
    \includegraphics[width=0.15\textwidth]{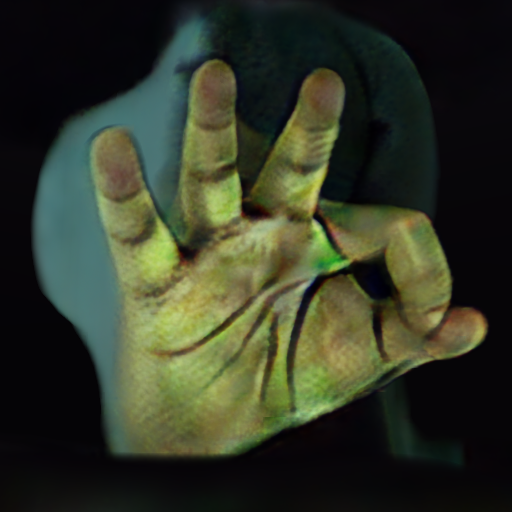} & 
    \includegraphics[width=0.15\textwidth]{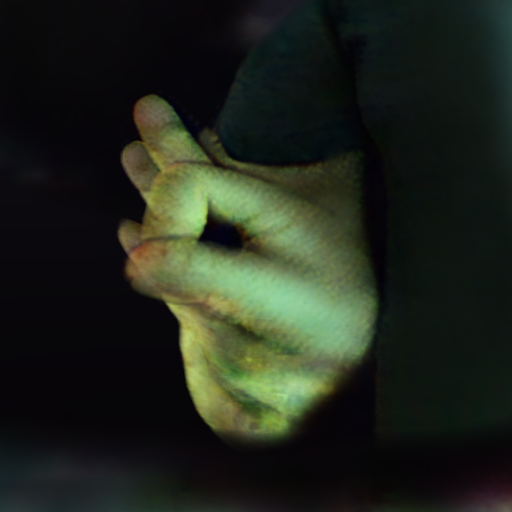} & 
    \includegraphics[width=0.15\textwidth]{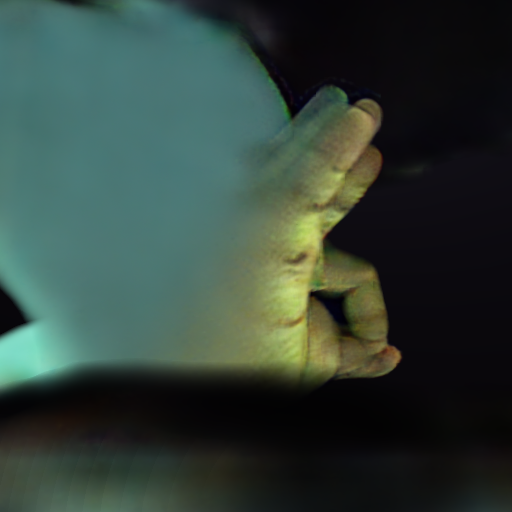} \\
    \rotatebox{90}{\hspace{1.0cm}\footnotesize Ours\;}&
    &
    \includegraphics[width=0.15\textwidth]{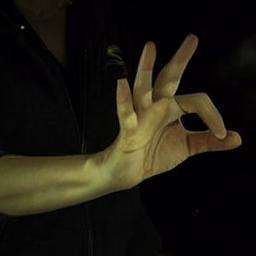} & 
    \includegraphics[width=0.15\textwidth]{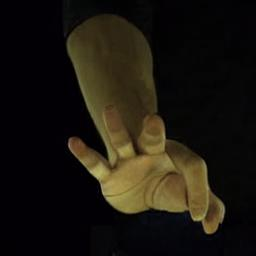} & 
    \includegraphics[width=0.15\textwidth]{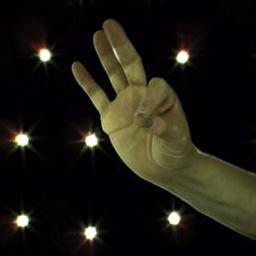} & 
    \includegraphics[width=0.15\textwidth]{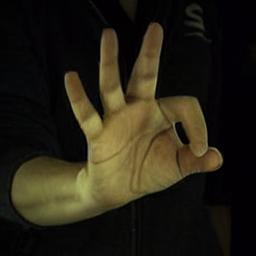} & 
    \includegraphics[width=0.15\textwidth]{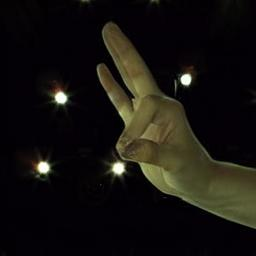} & 
    \includegraphics[width=0.15\textwidth]{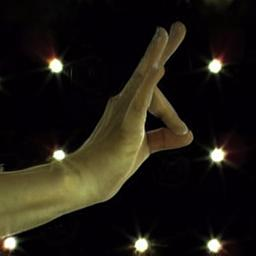} \\ 
    \rotatebox{90}{\hspace{1.0cm}\footnotesize GT\;}&
    &
    \includegraphics[width=0.15\textwidth]{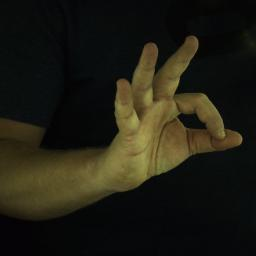} & 
    \includegraphics[width=0.15\textwidth]{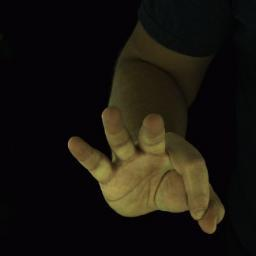} & 
    \includegraphics[width=0.15\textwidth]{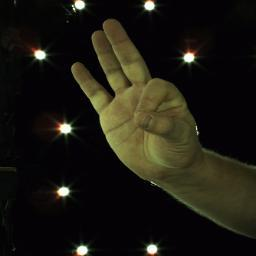} & 
    \includegraphics[width=0.15\textwidth]{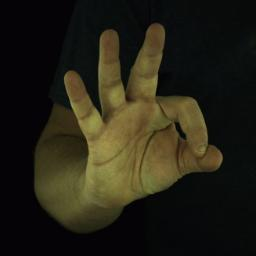} & 
    \includegraphics[width=0.15\textwidth]{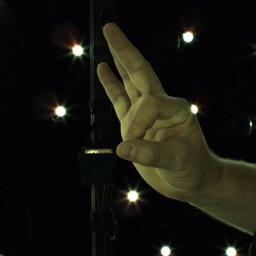} & 
    \includegraphics[width=0.15\textwidth]{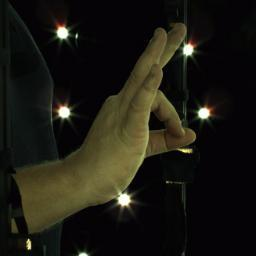} \\ [3.0pt]
    && View \#1 & View \#2 & View \#3 & View \#4 & View \#5 & View \#6\\
    \end{tabular}
    \caption{We test novel view synthesis (NVS) on the test data split of InterHand2.6M. Compared with baselines~\cite{zeronvs, imagedream} leveraging NeRF~\cite{nerf} to ensure 3D consistency, our geometry-free image generative model demonstrates great 3D understanding of hand. }
    \label{fig:suppl_nvs}
\end{figure*}

\begin{figure*}[!tp]

    \centering \footnotesize
    \begin{tabular}{ccccccccc}
    \rotatebox{90}{\hspace{1.1cm} \footnotesize\cite{zeronvs}} & 
    \; &
    \includegraphics[width=0.15\textwidth]{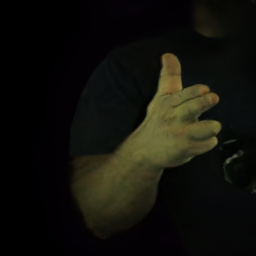} & 
    \includegraphics[width=0.15\textwidth]{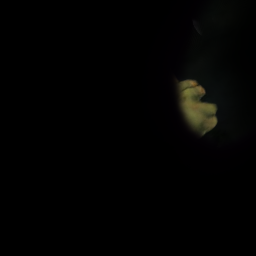} & 
    \includegraphics[width=0.15\textwidth]{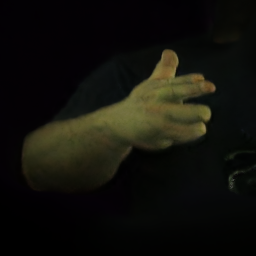} & 
    \includegraphics[width=0.15\textwidth]{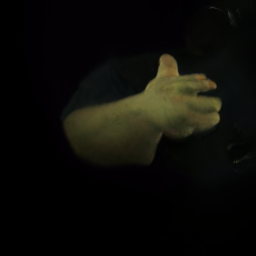} & 
    \includegraphics[width=0.15\textwidth]{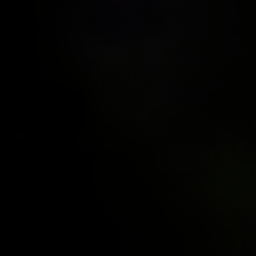} & 
    \includegraphics[width=0.15\textwidth]{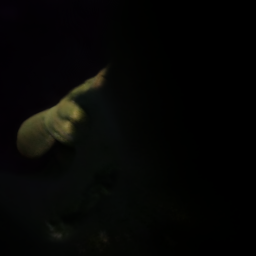} \\
    \rotatebox{90}{\hspace{1.3cm}\footnotesize \cite{imagedream}\;}&
    &
    \includegraphics[width=0.15\textwidth]{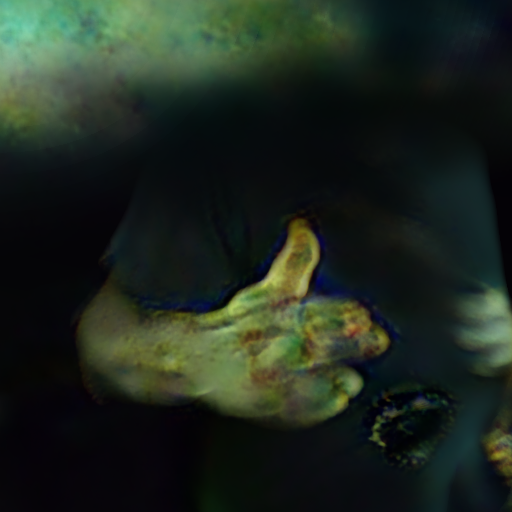} & 
    \includegraphics[width=0.15\textwidth]{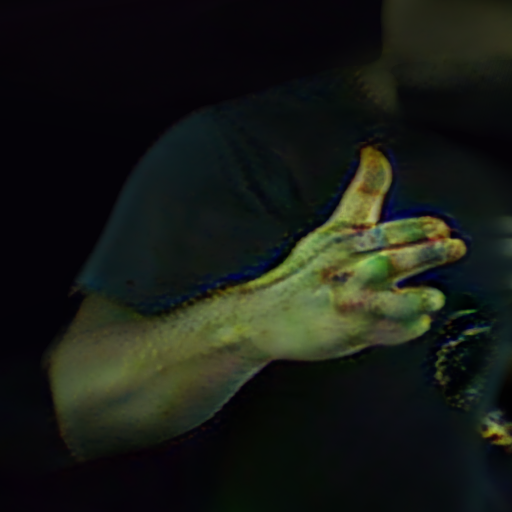} & 
    \includegraphics[width=0.15\textwidth]{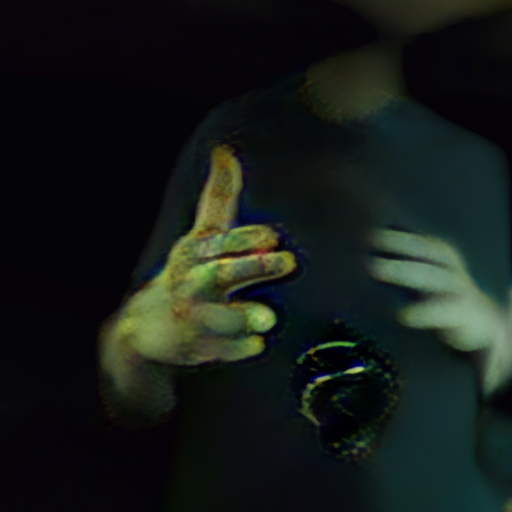} & 
    \includegraphics[width=0.15\textwidth]{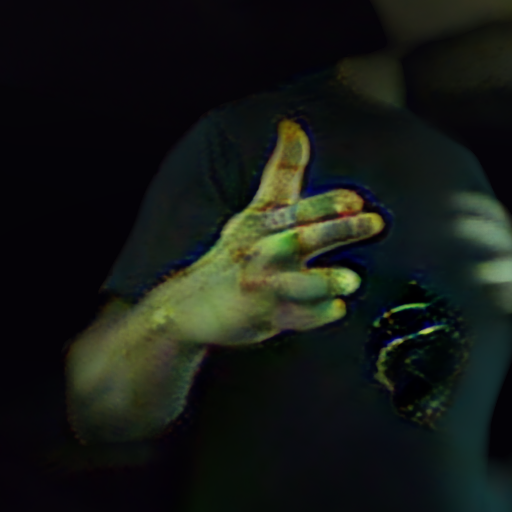} & 
    \includegraphics[width=0.15\textwidth]{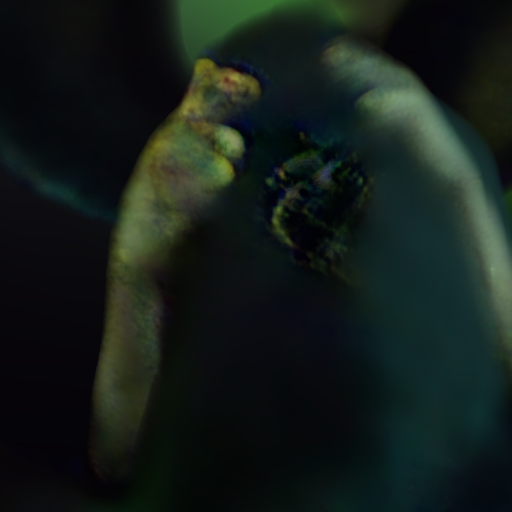} & 
    \includegraphics[width=0.15\textwidth]{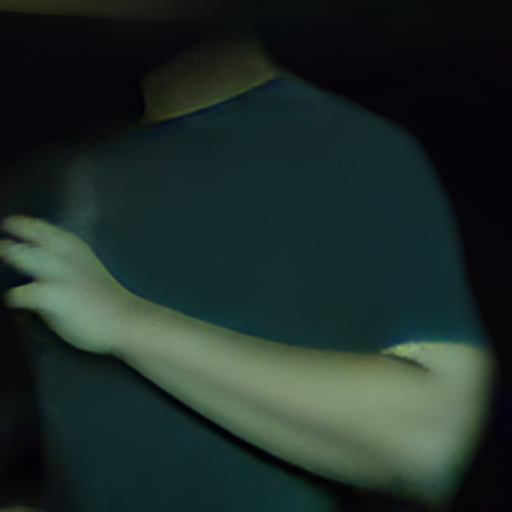} \\
    \rotatebox{90}{\hspace{1.2cm}\footnotesize Ours\;}&
    &
    \includegraphics[width=0.15\textwidth]{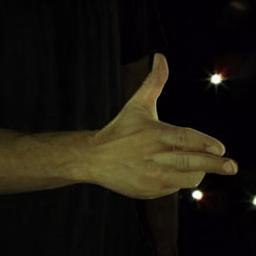} & 
    \includegraphics[width=0.15\textwidth]{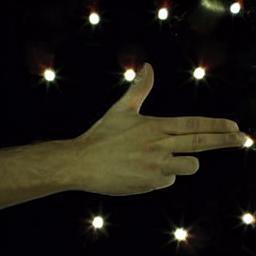} & 
    \includegraphics[width=0.15\textwidth]{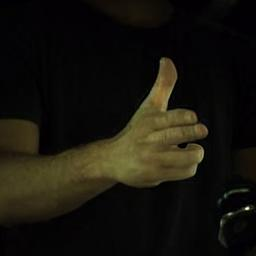} & 
    \includegraphics[width=0.15\textwidth]{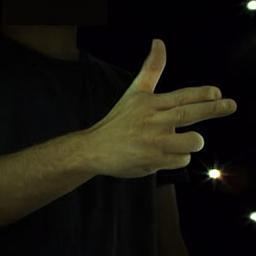} & 
    \includegraphics[width=0.15\textwidth]{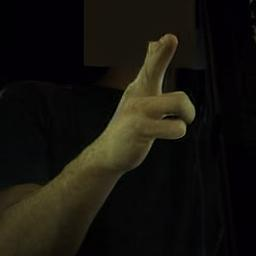} & 
    \includegraphics[width=0.15\textwidth]{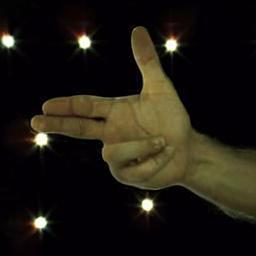} \\
    \rotatebox{90}{\hspace{1.2cm}\footnotesize GT\;}&
    &
    \includegraphics[width=0.15\textwidth]{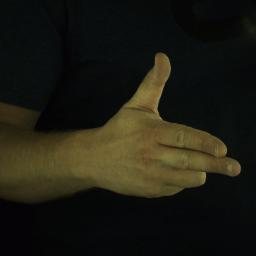} & 
    \includegraphics[width=0.15\textwidth]{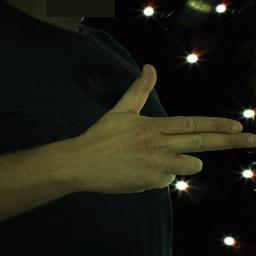} & 
    \includegraphics[width=0.15\textwidth]{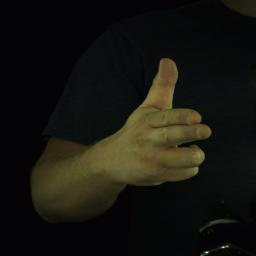} & 
    \includegraphics[width=0.15\textwidth]{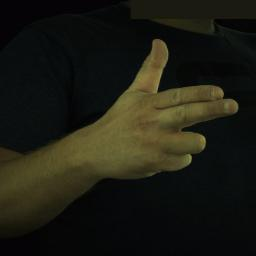} & 
    \includegraphics[width=0.15\textwidth]{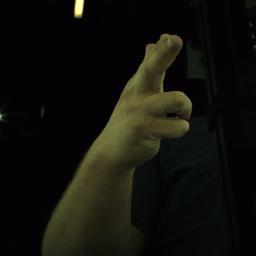} & 
    \includegraphics[width=0.15\textwidth]{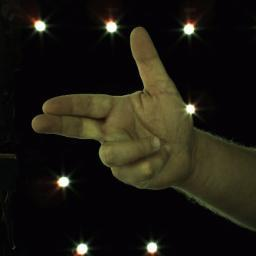} \\[3.0pt]
    \rotatebox{90}{\hspace{1.0cm} \footnotesize\cite{zeronvs}} & 
    \; &
    \includegraphics[width=0.15\textwidth]{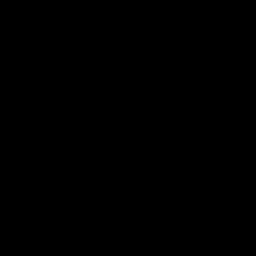} & 
    \includegraphics[width=0.15\textwidth]{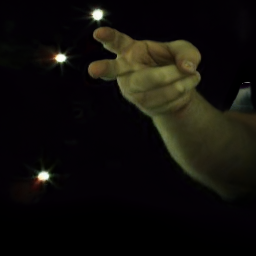} & 
    \includegraphics[width=0.15\textwidth]{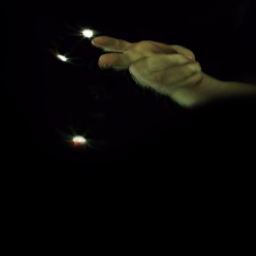} & 
    \includegraphics[width=0.15\textwidth]{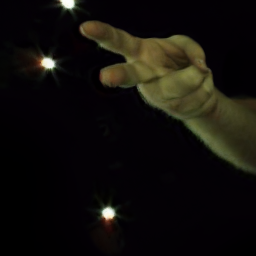} & 
    \includegraphics[width=0.15\textwidth]{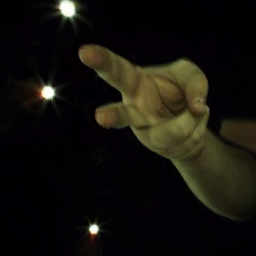} & 
    \includegraphics[width=0.15\textwidth]{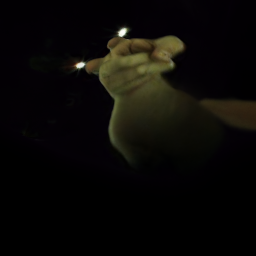} \\
    \rotatebox{90}{\hspace{1.0cm}\footnotesize \cite{imagedream}\;}&
    &
    \includegraphics[width=0.15\textwidth]{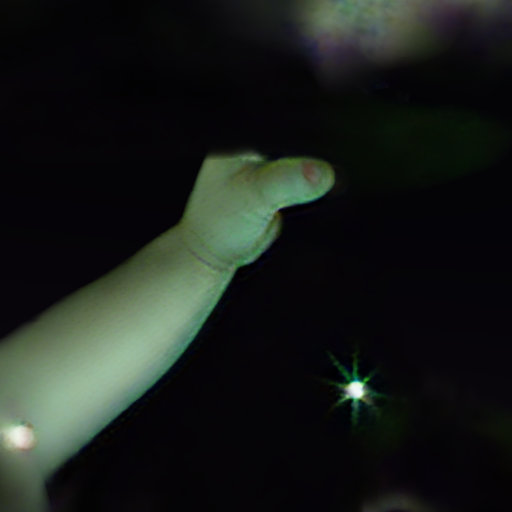} & 
    \includegraphics[width=0.15\textwidth]{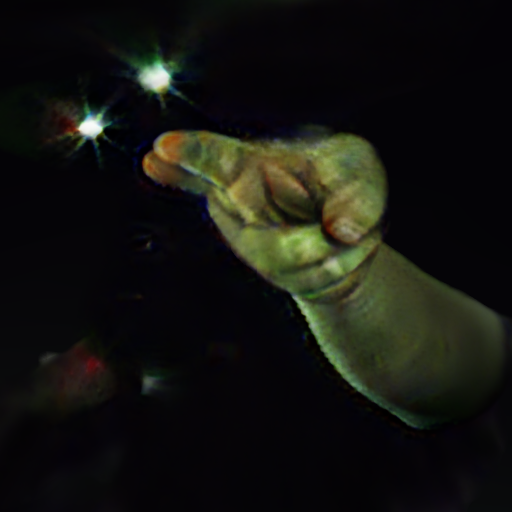} & 
    \includegraphics[width=0.15\textwidth]{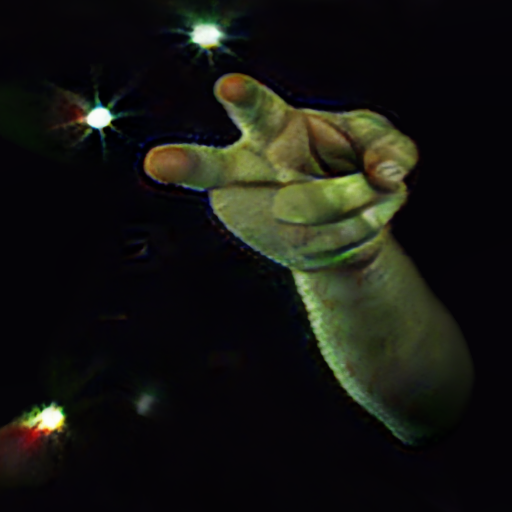} & 
    \includegraphics[width=0.15\textwidth]{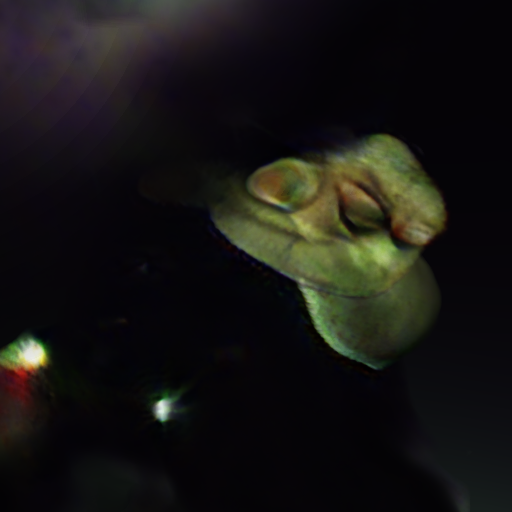} & 
    \includegraphics[width=0.15\textwidth]{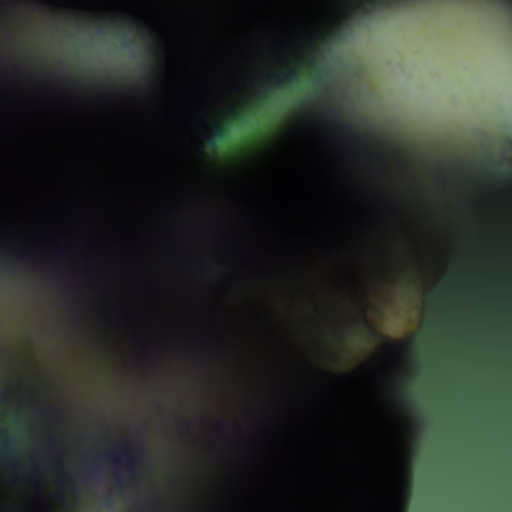} & 
    \includegraphics[width=0.15\textwidth]{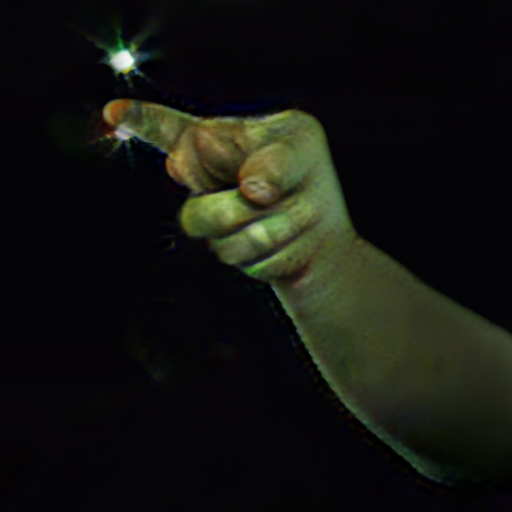} \\
    \rotatebox{90}{\hspace{1.0cm}\footnotesize Ours\;}&
    &
    \includegraphics[width=0.15\textwidth]{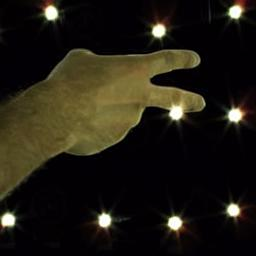} & 
    \includegraphics[width=0.15\textwidth]{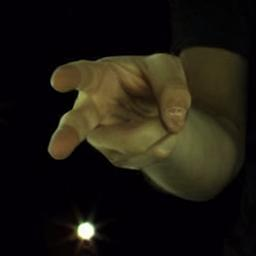} & 
    \includegraphics[width=0.15\textwidth]{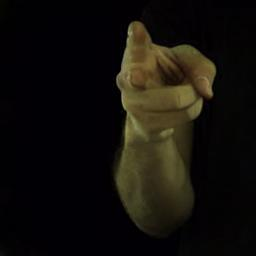} & 
    \includegraphics[width=0.15\textwidth]{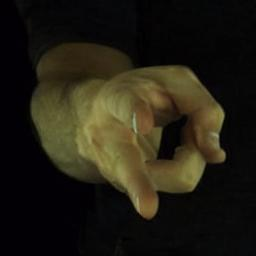} & 
    \includegraphics[width=0.15\textwidth]{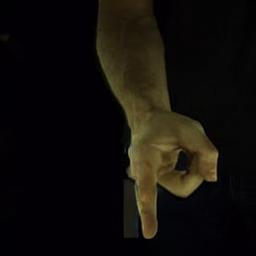} & 
    \includegraphics[width=0.15\textwidth]{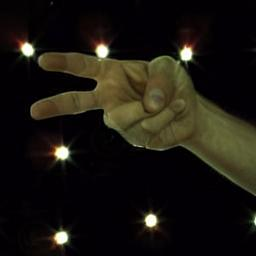} \\ 
    \rotatebox{90}{\hspace{1.0cm}\footnotesize GT\;}&
    &
    \includegraphics[width=0.15\textwidth]{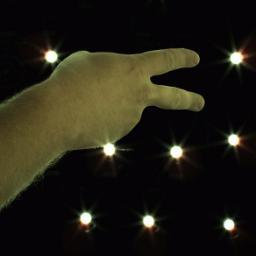} & 
    \includegraphics[width=0.15\textwidth]{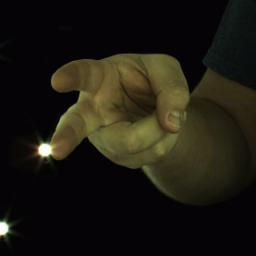} & 
    \includegraphics[width=0.15\textwidth]{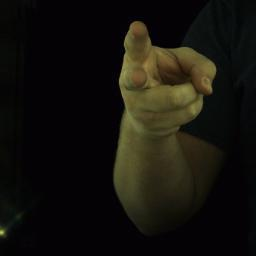} & 
    \includegraphics[width=0.15\textwidth]{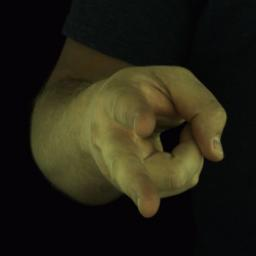} & 
    \includegraphics[width=0.15\textwidth]{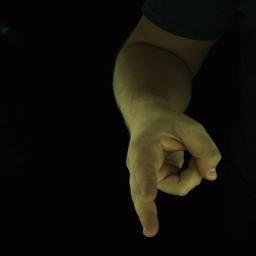} & 
    \includegraphics[width=0.15\textwidth]{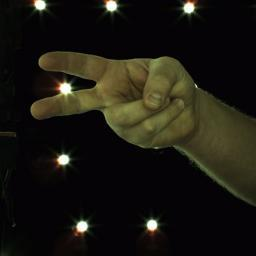} \\ [3.0pt]
    && View \#1 & View \#2 & View \#3 & View \#4 & View \#5 & View \#6\\
    \end{tabular}
    \caption{Fig.~\ref{fig:suppl_nvs} continued.}
    \label{fig:suppl_nvs2}
\end{figure*}

% NVS in-the-wild

\begin{figure*}[!tp]

    \centering \footnotesize
    \begin{tabular}{cccccc}
    % \rotatebox{90}{\hspace{1.0cm} Reference} & 
    % \; &
    \includegraphics[width=0.15\textwidth]{figs/nvs/in-the-wild/five/reference.jpg} & 
    \includegraphics[width=0.15\textwidth]{figs/nvs/in-the-wild/five/five (1).jpg} & 
    \includegraphics[width=0.15\textwidth]{figs/nvs/in-the-wild/five/five (2).jpg} & 
    \includegraphics[width=0.15\textwidth]{figs/nvs/in-the-wild/five/five (3).jpg} & 
    \includegraphics[width=0.15\textwidth]{figs/nvs/in-the-wild/five/five (4).jpg} & 
    \includegraphics[width=0.15\textwidth]{figs/nvs/in-the-wild/five/five (5).jpg} \\
    \includegraphics[width=0.15\textwidth]{figs/nvs/in-the-wild/okay/reference.jpg} & 
    \includegraphics[width=0.15\textwidth]{figs/nvs/in-the-wild/okay/okay (1).jpg} & 
    \includegraphics[width=0.15\textwidth]{figs/nvs/in-the-wild/okay/okay (2).jpg} & 
    \includegraphics[width=0.15\textwidth]{figs/nvs/in-the-wild/okay/okay (3).jpg} & 
    \includegraphics[width=0.15\textwidth]{figs/nvs/in-the-wild/okay/okay (4).jpg} & 
    \includegraphics[width=0.15\textwidth]{figs/nvs/in-the-wild/okay/okay (5).jpg} \\
    \includegraphics[width=0.15\textwidth]{figs/nvs/in-the-wild/three/reference.jpg} & 
    \includegraphics[width=0.15\textwidth]{figs/nvs/in-the-wild/three/three (1).jpg} & 
    \includegraphics[width=0.15\textwidth]{figs/nvs/in-the-wild/three/three (2).jpg} & 
    \includegraphics[width=0.15\textwidth]{figs/nvs/in-the-wild/three/three (3).jpg} & 
    \includegraphics[width=0.15\textwidth]{figs/nvs/in-the-wild/three/three (4).jpg} & 
    \includegraphics[width=0.15\textwidth]{figs/nvs/in-the-wild/three/three (5).jpg} \\[2.0pt]
    Reference& View \#1 & View \#2 & View \#3 & View \#4 & View\#5\\
    \end{tabular}
    \vspace{-0.2cm}
    \caption{Internet-sourced single image to Novel View Synthesis. \modelname can provide reasonable novel view synthesis, showing robust 3D piror of hand without explicit 3D geometric context such as depth or mesh template.}
    \label{fig:suppl_nvs_itw}
\end{figure*}

% HOI

\begin{figure*}[!tp]

    \centering \footnotesize
    \begin{tabular}{cccccccc}
    \rotatebox{90}{\hspace{0.6cm} \footnotesize CosHand~\cite{coshand}} & 
    \; &
    \includegraphics[width=0.16\textwidth]{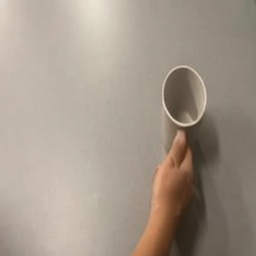} & 
    \includegraphics[width=0.16\textwidth]{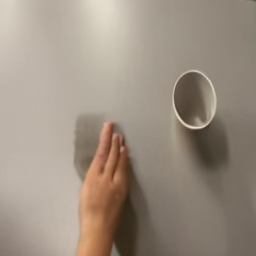} & 
    \includegraphics[width=0.16\textwidth]{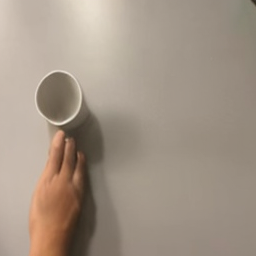} & 
    \includegraphics[width=0.16\textwidth]{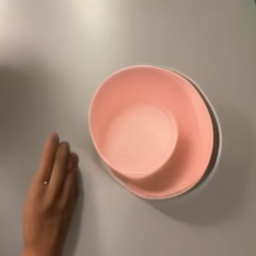} & 
    \includegraphics[width=0.16\textwidth]{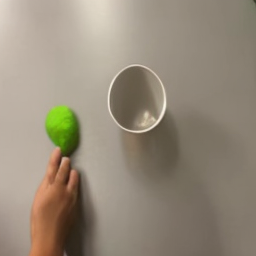} \\
    \rotatebox{90}{\hspace{1.2cm}\footnotesize Ours}&
    &
    \includegraphics[width=0.16\textwidth]{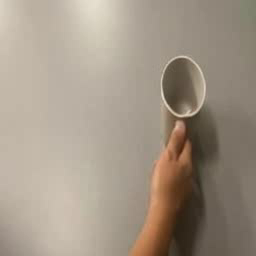} & 
    \includegraphics[width=0.16\textwidth]{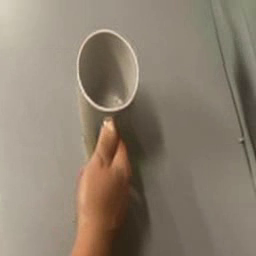} & 
    \includegraphics[width=0.16\textwidth]{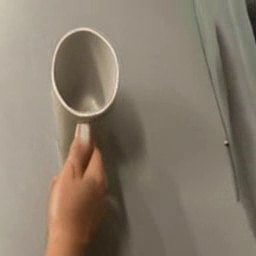} & 
    \includegraphics[width=0.16\textwidth]{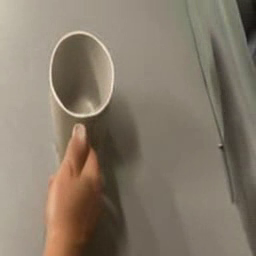} & 
    \includegraphics[width=0.16\textwidth]{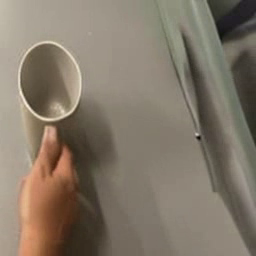} \\
    \rotatebox{90}{\hspace{0.6cm}\footnotesize CosHand~\cite{coshand}}&
    &
    \includegraphics[width=0.16\textwidth]{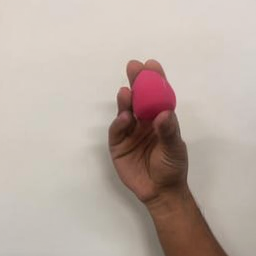} & 
    \includegraphics[width=0.16\textwidth]{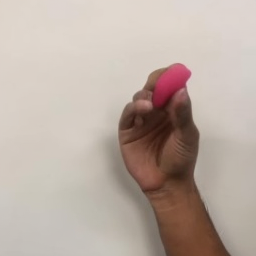} & 
    \includegraphics[width=0.16\textwidth]{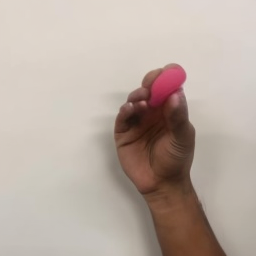} & 
    \includegraphics[width=0.16\textwidth]{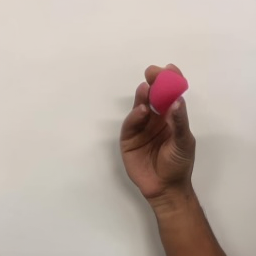} & 
    \includegraphics[width=0.16\textwidth]{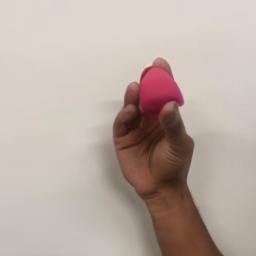} \\
    \rotatebox{90}{\hspace{1.2cm}\footnotesize Ours}&
    &
    \includegraphics[width=0.16\textwidth]{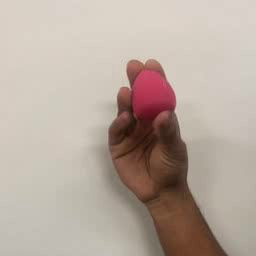} & 
    \includegraphics[width=0.16\textwidth]{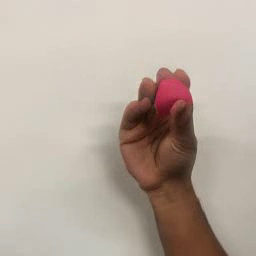} & 
    \includegraphics[width=0.16\textwidth]{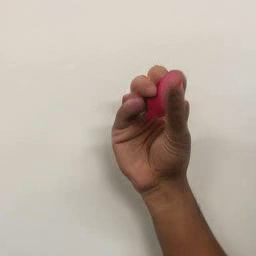} & 
    \includegraphics[width=0.16\textwidth]{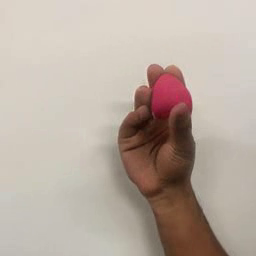} & 
    \includegraphics[width=0.16\textwidth]{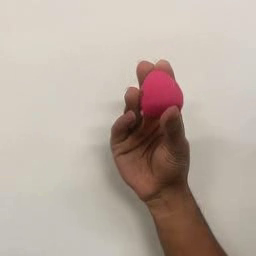} \\ [4.0pt] 
    && Reference& \multicolumn{4}{c}{Time} \vspace{.5em}\\
    &&& \multicolumn{4}{c}{
        \begin{tikzpicture}
            \draw[->, line width=0.3mm] (0,0) -- (9.5,0);
        \end{tikzpicture}} \\
    \end{tabular}
    \caption{\modelname has naturally seen many hand-object interaction and manipulation scenes and surprisingly develops emergent physical understanding of HOI (object translation and deformation.) without explicit knowledge of the object context. On the other hand, CosHand~\cite{coshand} is trained on specific HOI data focusing on interaction-induced change but shows some overfitting (1st row).}
    \label{fig:suppl_hoi}
\end{figure*}

% Fixing Hand

\begin{figure*}[!tp]

    \centering \footnotesize
    \begin{tabular}{cccc}
        \includegraphics[width=0.175\textwidth]{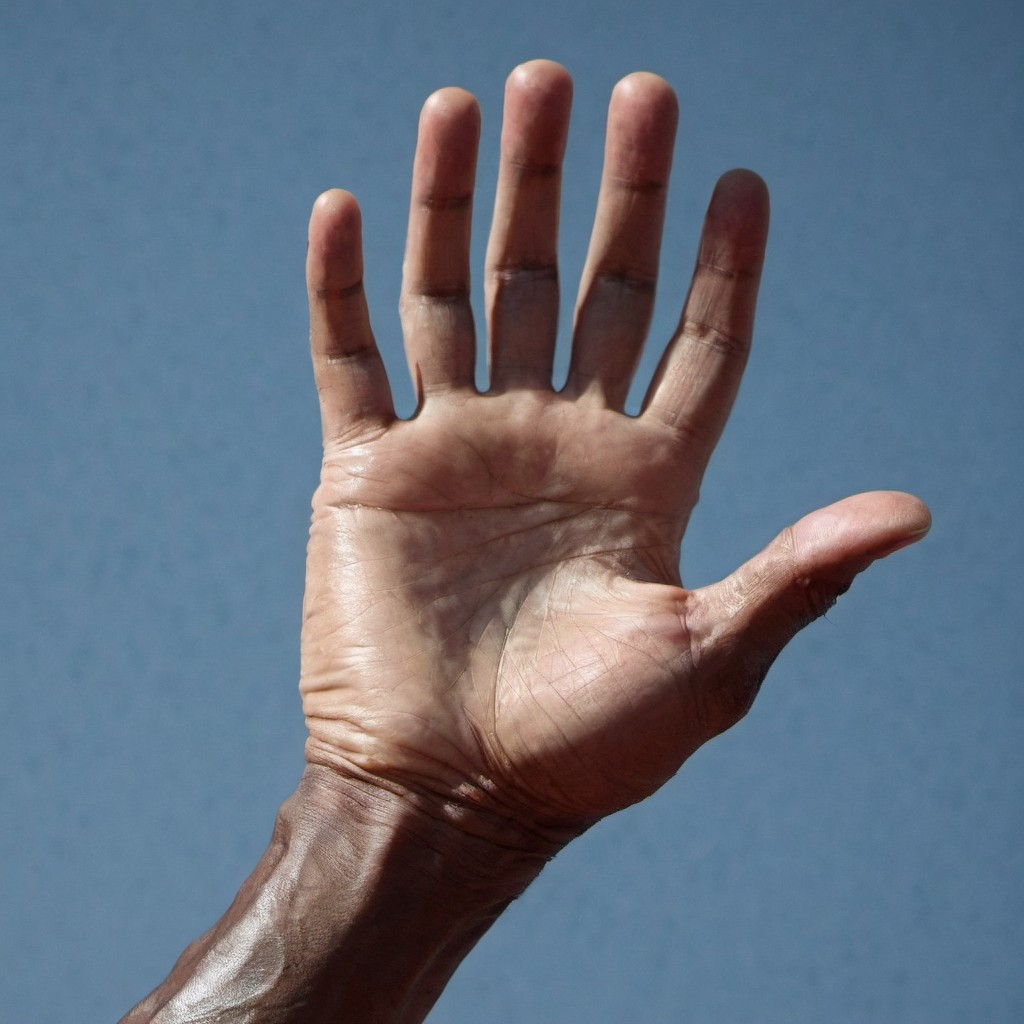} & 
        \includegraphics[width=0.175\textwidth]{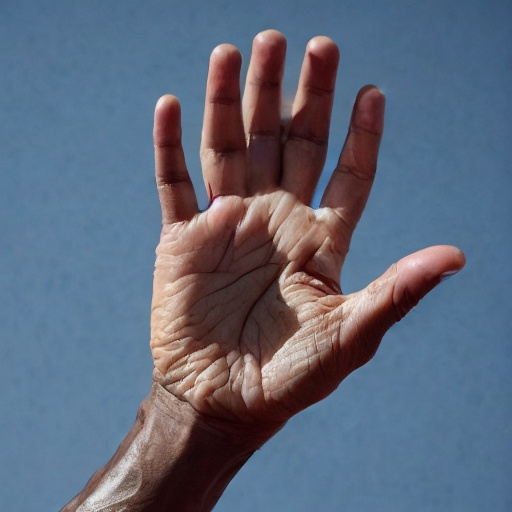} & 
        \includegraphics[width=0.175\textwidth]{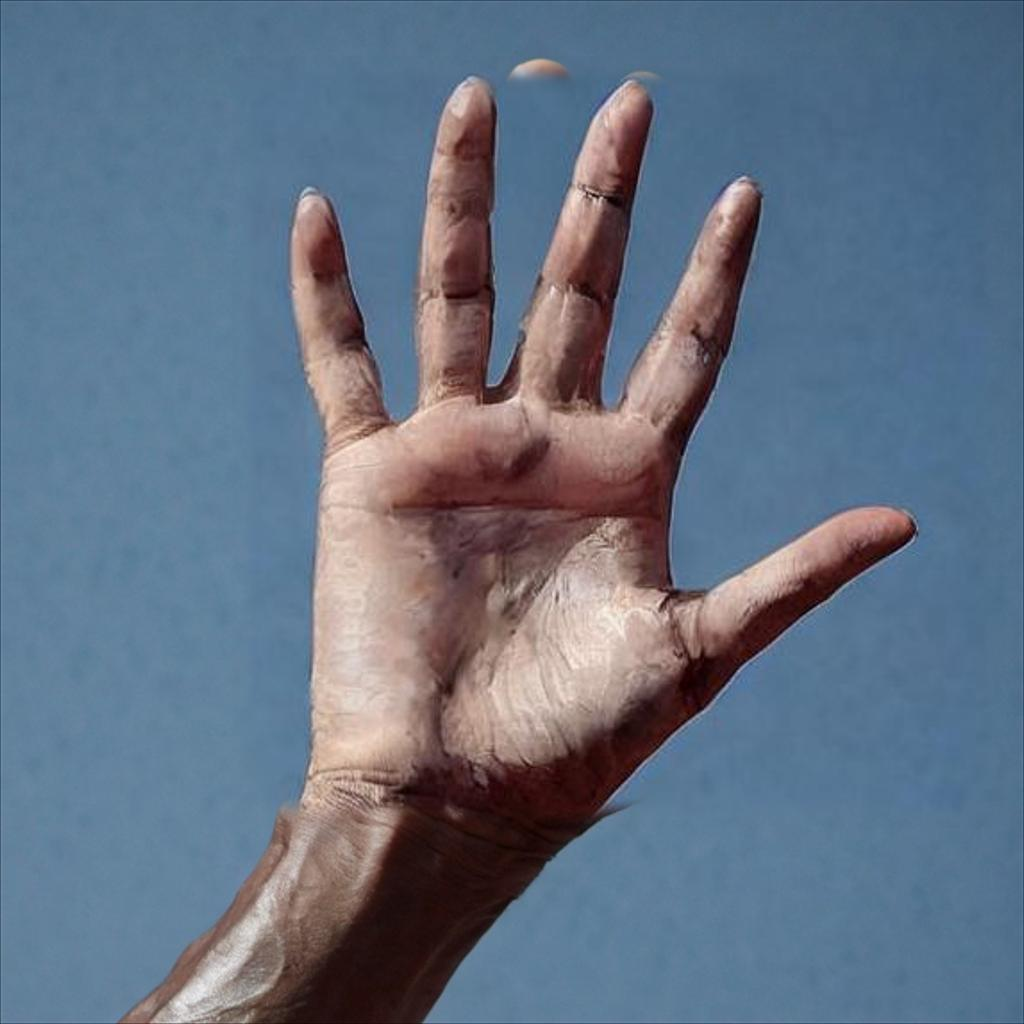} & 
        \includegraphics[width=0.175\textwidth]{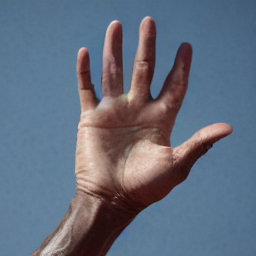} \\
        \includegraphics[width=0.175\textwidth]{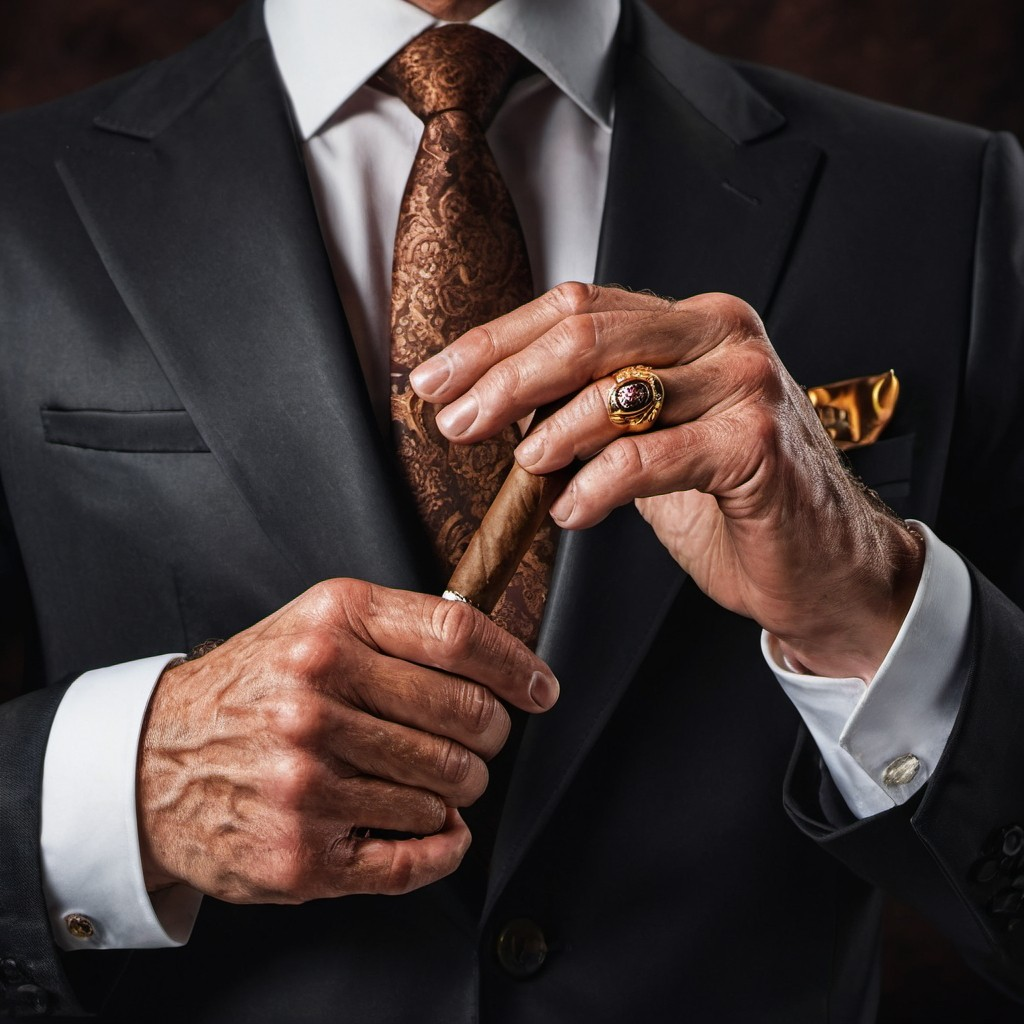} & 
        \includegraphics[width=0.175\textwidth]{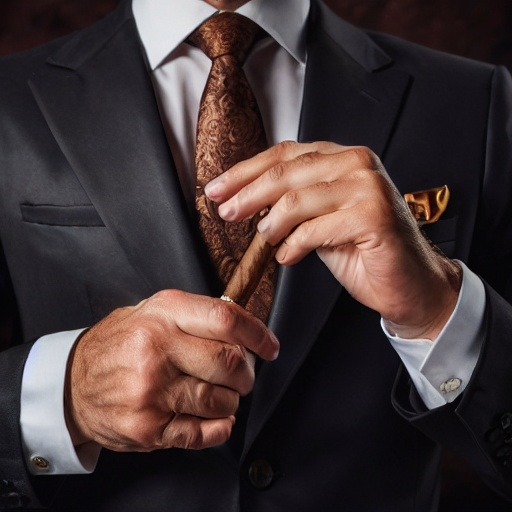} & 
        \includegraphics[width=0.175\textwidth]{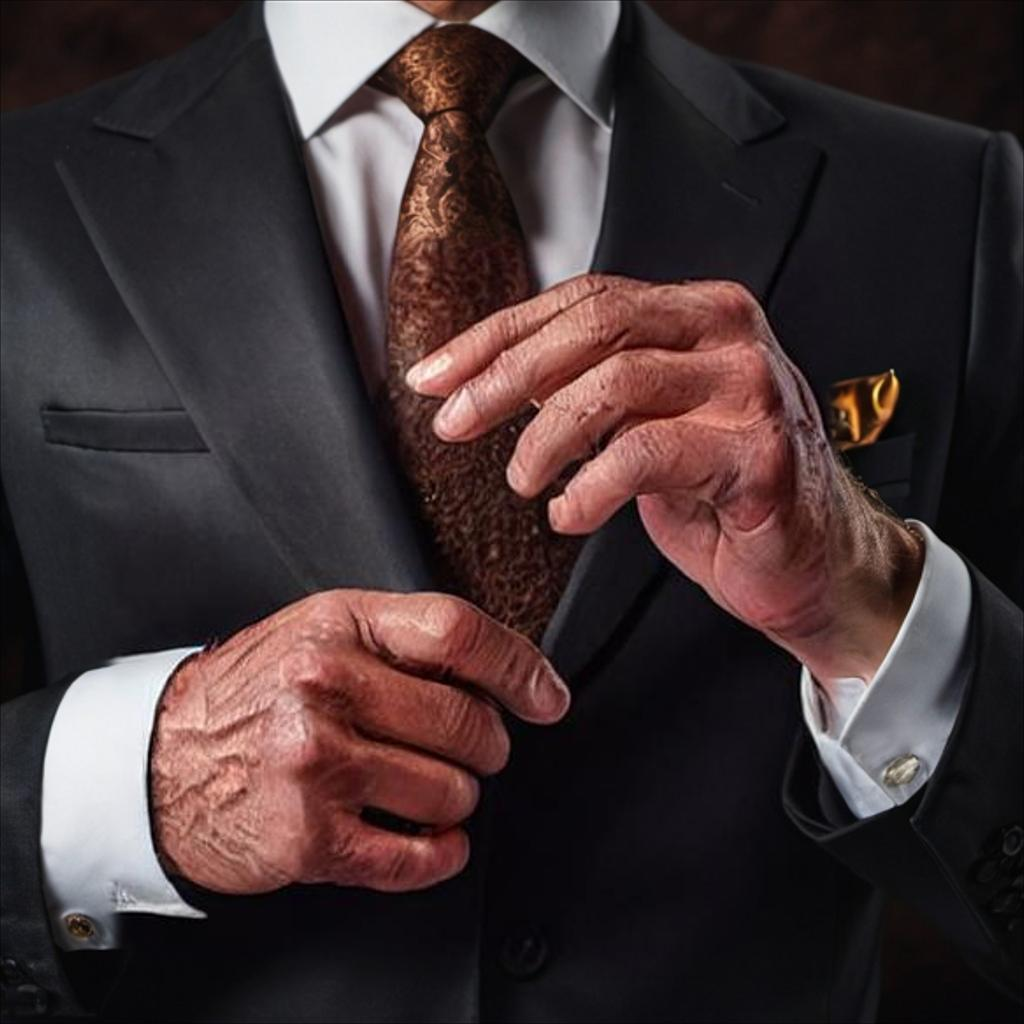} & 
        \includegraphics[width=0.175\textwidth]{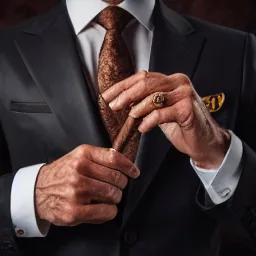} \\
        \includegraphics[width=0.175\textwidth]{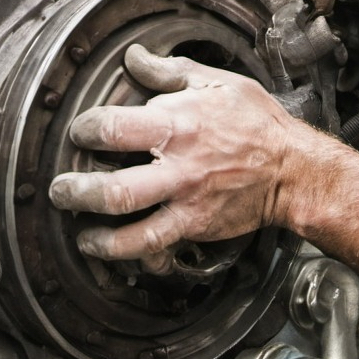} & 
        \includegraphics[width=0.175\textwidth]{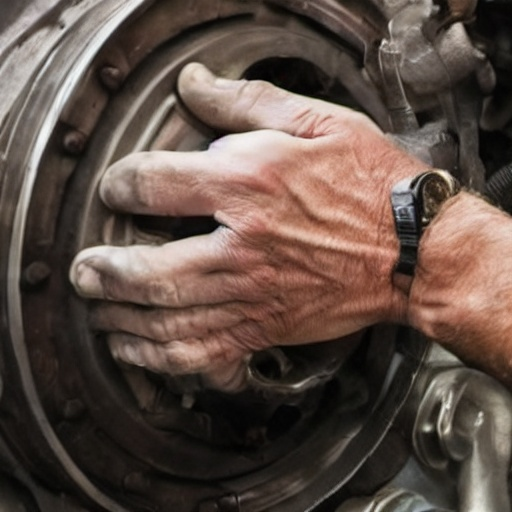} & 
        \includegraphics[width=0.175\textwidth]{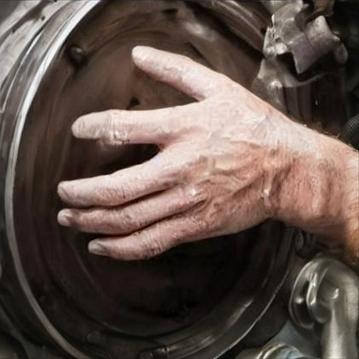} & 
        \includegraphics[width=0.175\textwidth]{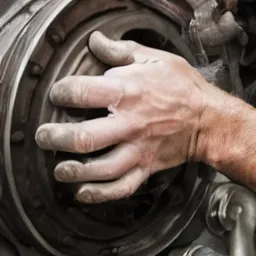} \\ 
        \includegraphics[width=0.175\textwidth]{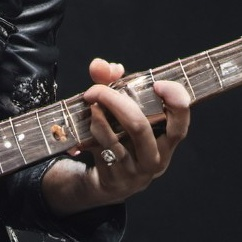} & 
        \includegraphics[width=0.175\textwidth]{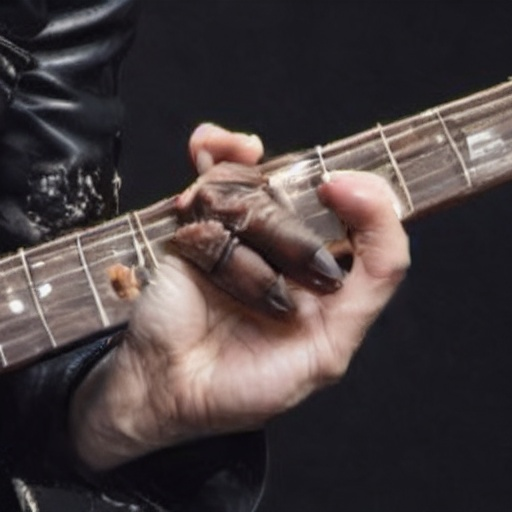} & 
        \includegraphics[width=0.175\textwidth]{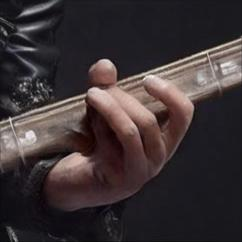} & 
        \includegraphics[width=0.175\textwidth]{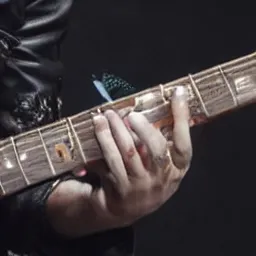} \\ 
        \includegraphics[width=0.175\textwidth]{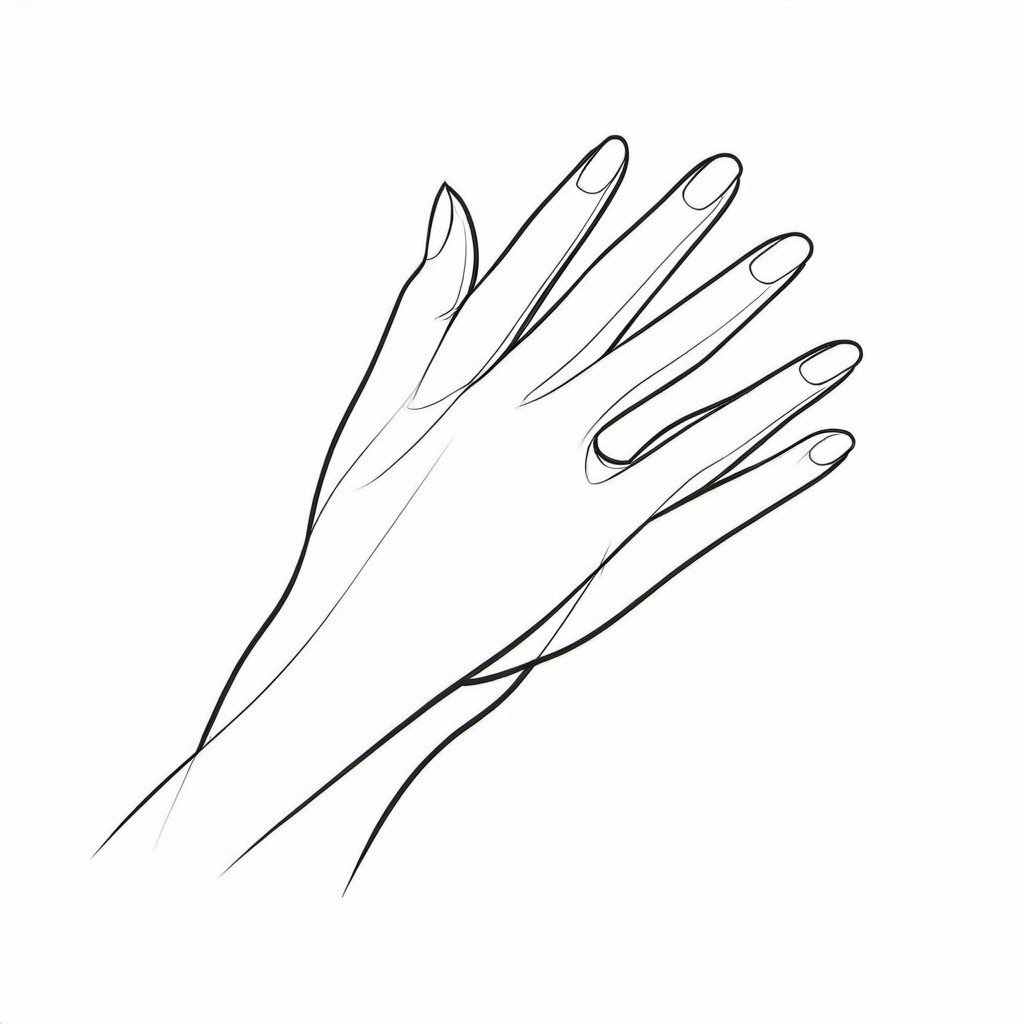} & 
        \includegraphics[width=0.175\textwidth]{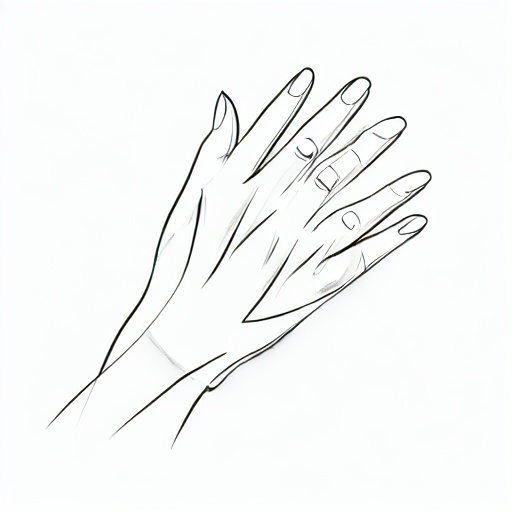} & 
        \includegraphics[width=0.175\textwidth]{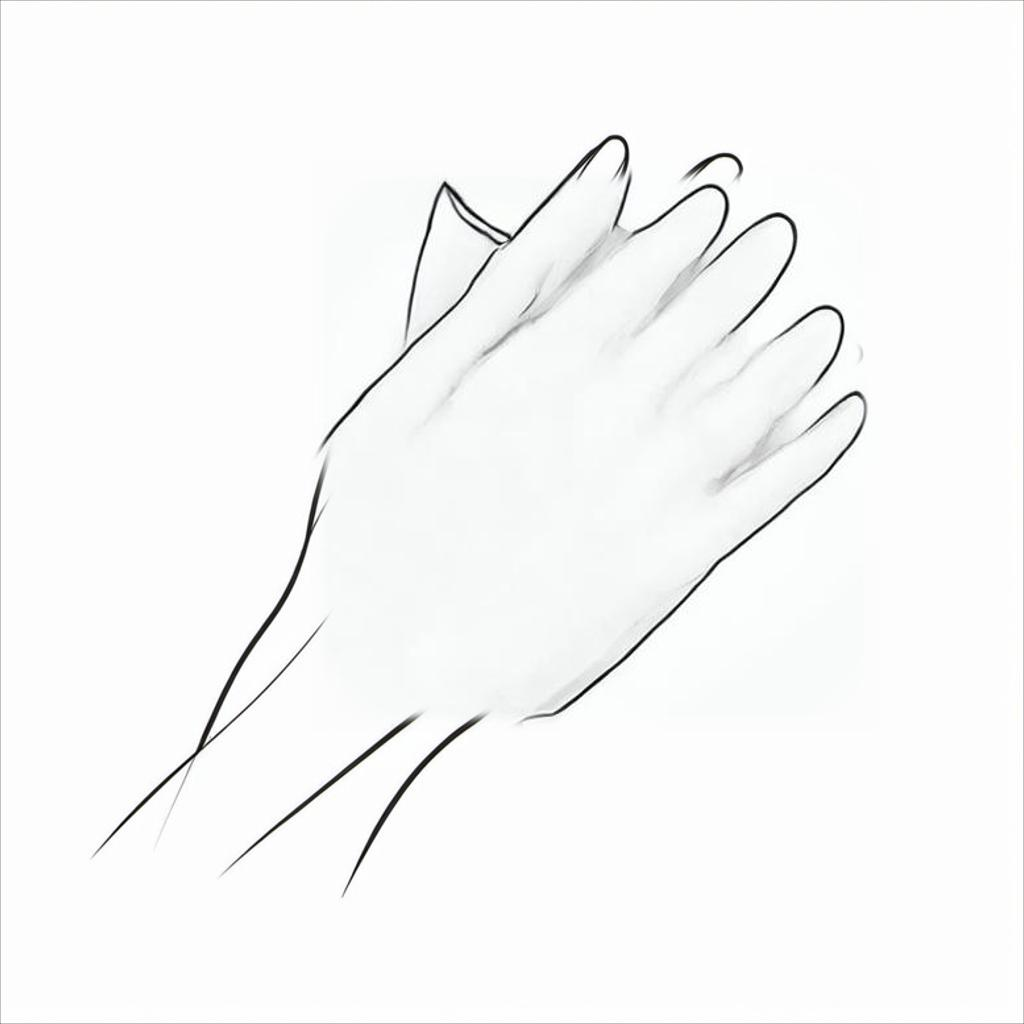} & 
        \includegraphics[width=0.175\textwidth]{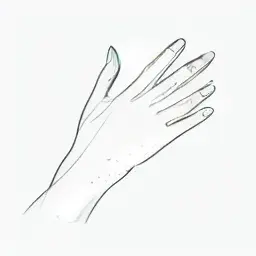} \\ 
        \includegraphics[width=0.175\textwidth]{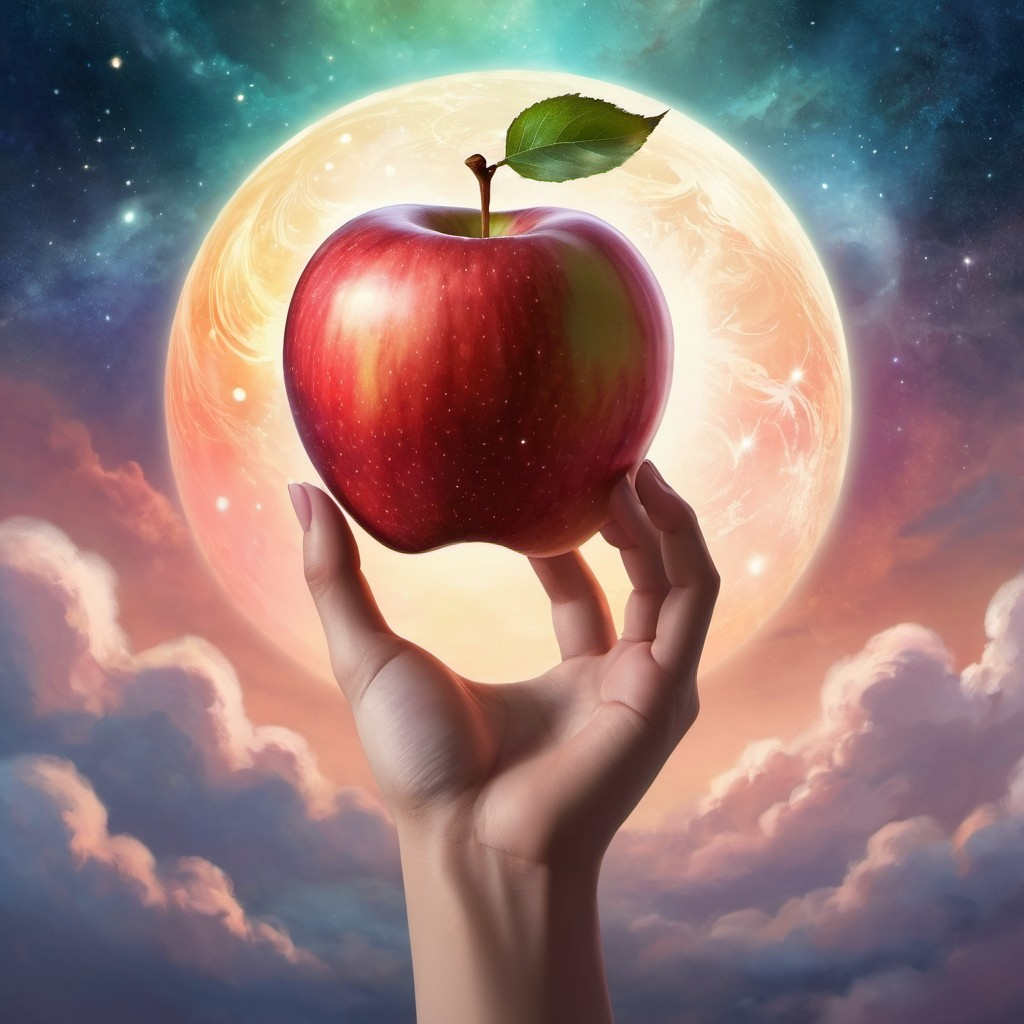} & 
        \includegraphics[width=0.175\textwidth]{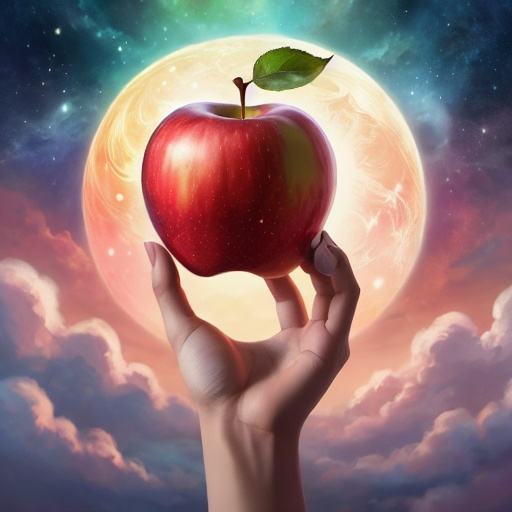} & 
        \includegraphics[width=0.175\textwidth]{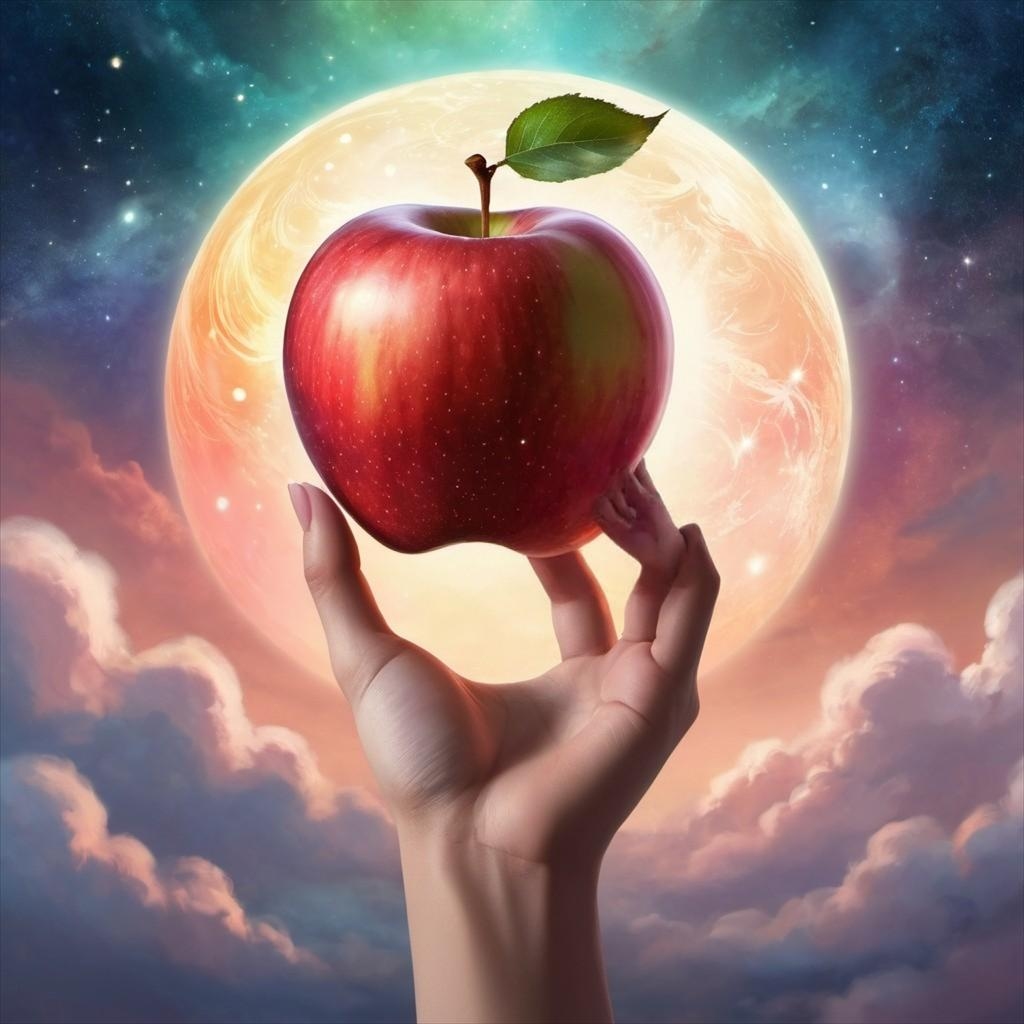} & 
        \includegraphics[width=0.175\textwidth]{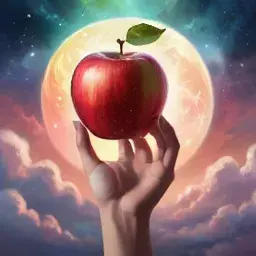} \\ 
        \includegraphics[width=0.175\textwidth]{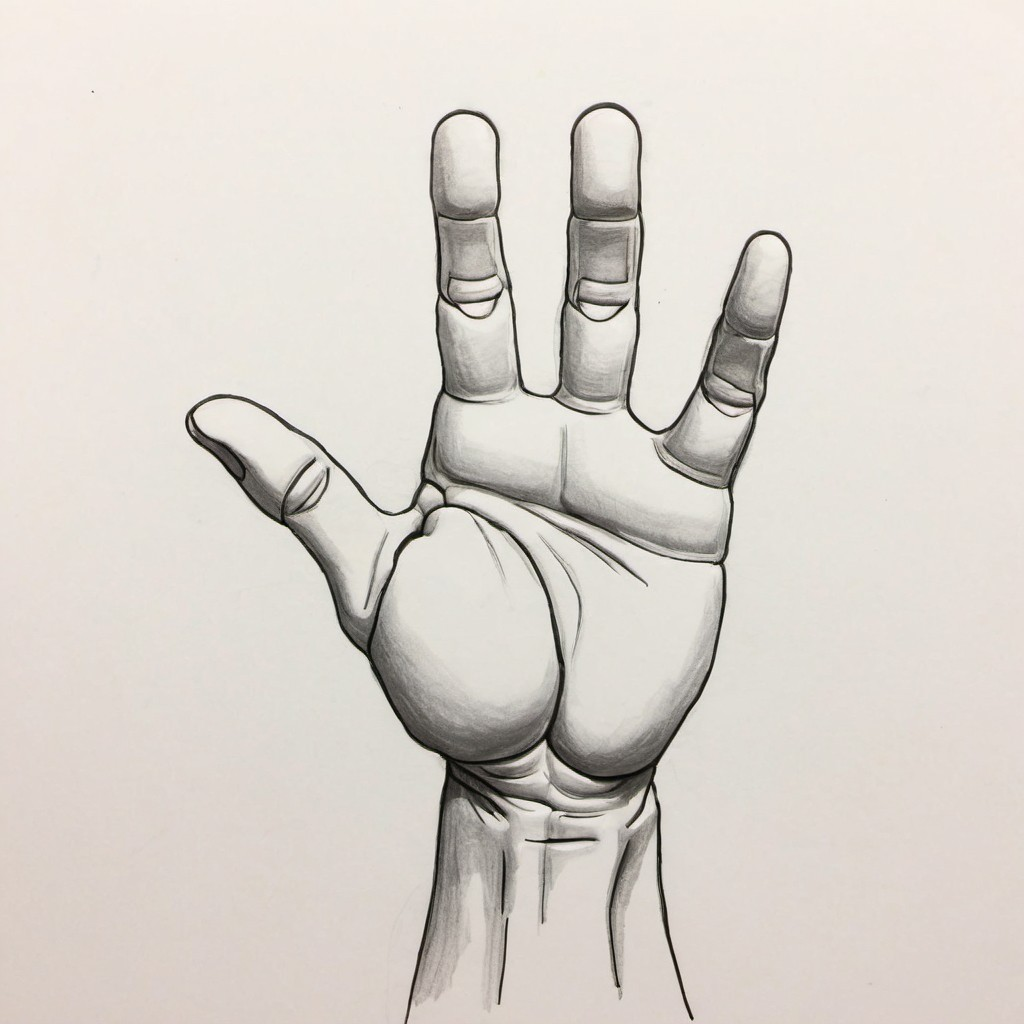} & 
        \includegraphics[width=0.175\textwidth]{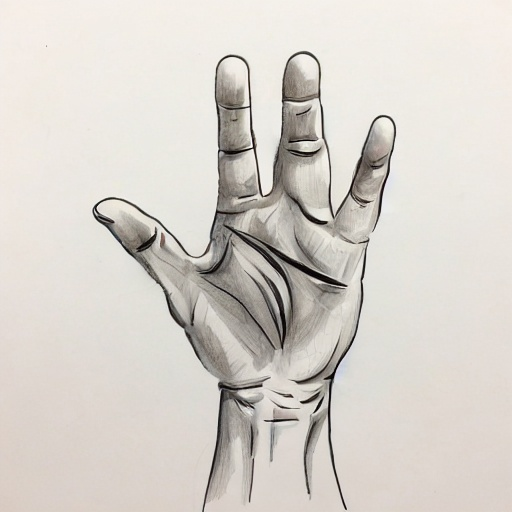}&        
        \includegraphics[width=0.175\textwidth]{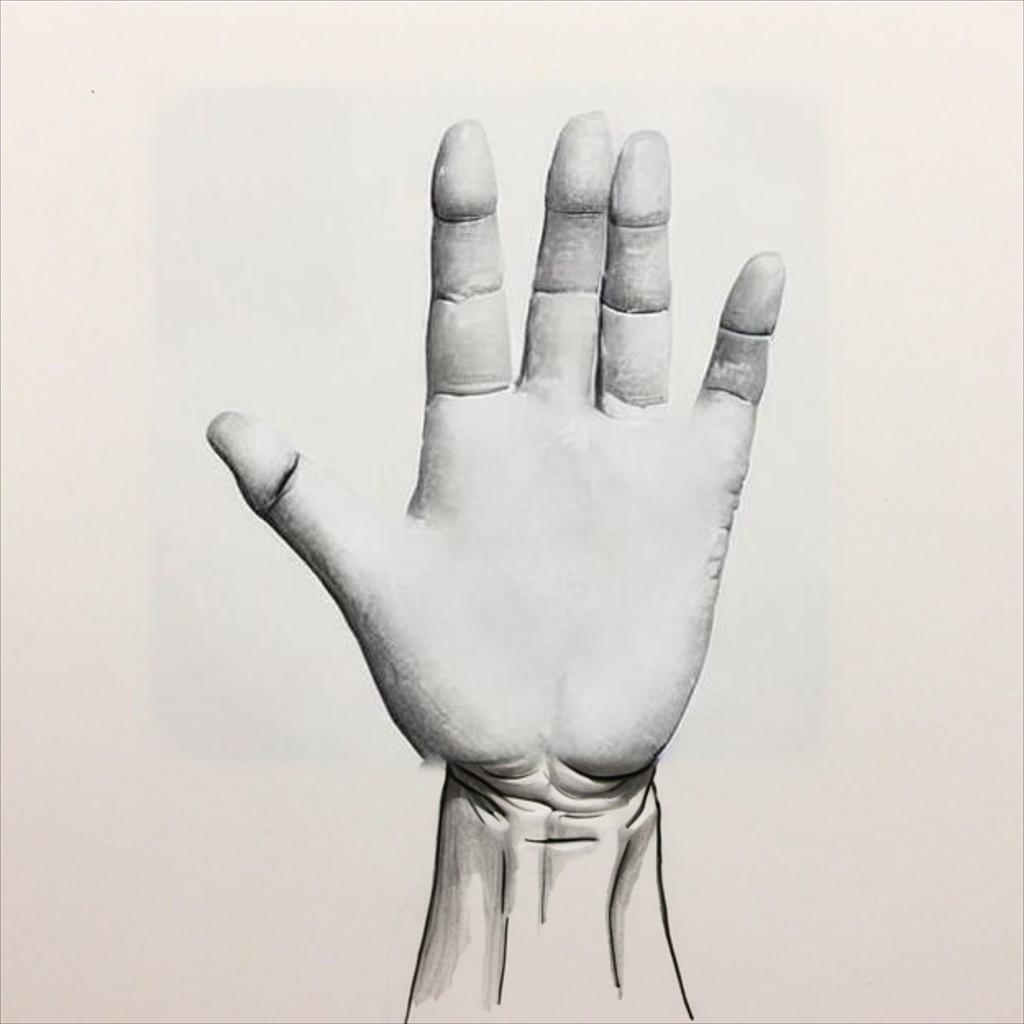} &
        \includegraphics[width=0.175\textwidth]{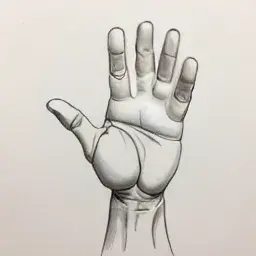}\\[1.0pt]
        Malformed & ~\cite{lu2023handrefiner} &~\cite{realishuman} & Ours \\
    \end{tabular}
    \vspace{-0.3cm}
    \caption{Compared with task-specific methods like HandRefiner~\cite{lu2023handrefiner} and RealisHuman~\cite{realishuman} which requires accurate 3D hand estimation, our \modelname performs zero-shot hand fixing, demonstrating exceptional generalization to diverse artistic and abstract styles (5th and 7th row). Our model also shows better understanding of the context, particularly preserving the hand-object interaction context after fixing the hand (2nd, 4th, and 6th row). }
    \label{fig:suppl_fixhands}
\end{figure*}

% Video Synthesis

\begin{figure*}[!tp]

    \centering \footnotesize
    \begin{tabular}{cccccccccc}
    \rotatebox{90}{\hspace{1.0cm} \footnotesize\cite{controlnext}} & 
    \; &
    \includegraphics[width=0.13\textwidth]{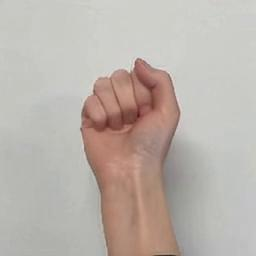} & 
    \includegraphics[width=0.13\textwidth]{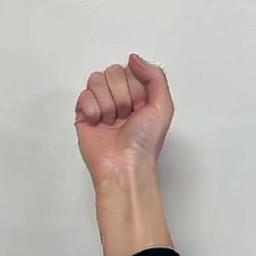} & 
    \includegraphics[width=0.13\textwidth]{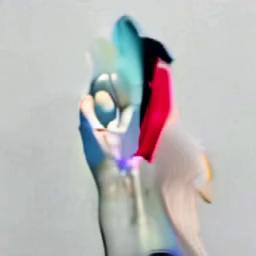} & 
    \includegraphics[width=0.13\textwidth]{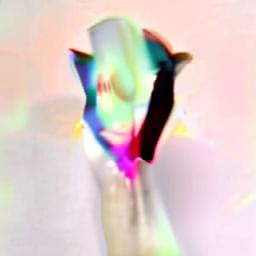} & 
    \includegraphics[width=0.13\textwidth]{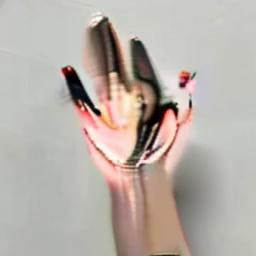} &
    \includegraphics[width=0.13\textwidth]{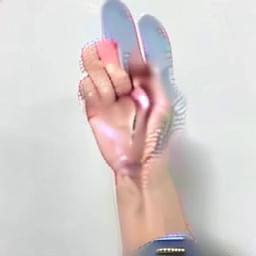} &
    \includegraphics[width=0.13\textwidth]{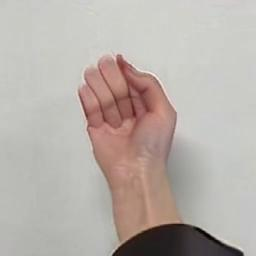} \\
    \rotatebox{90}{\hspace{1.0cm}\footnotesize \cite{animate_anyone}\;}&
    &
    \includegraphics[width=0.13\textwidth]{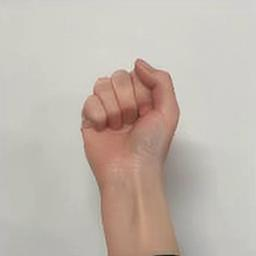} & 
    \includegraphics[width=0.13\textwidth]{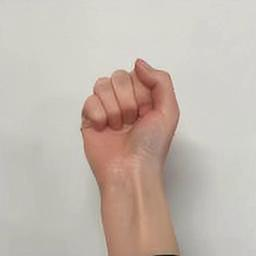} & 
    \includegraphics[width=0.13\textwidth]{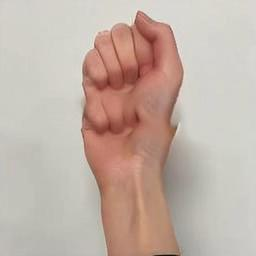} & 
    \includegraphics[width=0.13\textwidth]{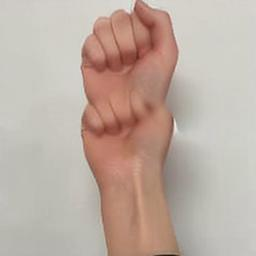} & 
    \includegraphics[width=0.13\textwidth]{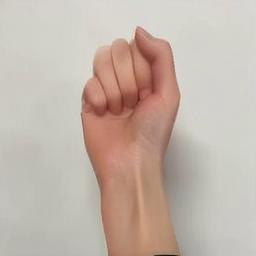} &
    \includegraphics[width=0.13\textwidth]{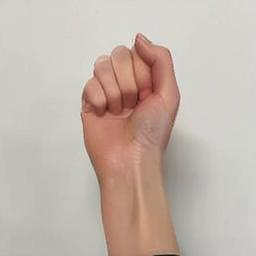} &
    \includegraphics[width=0.13\textwidth]{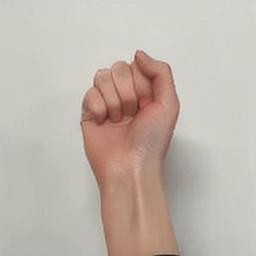} \\
    \rotatebox{90}{\hspace{1.0cm}\footnotesize Ours\;}&
    &
    \includegraphics[width=0.13\textwidth]{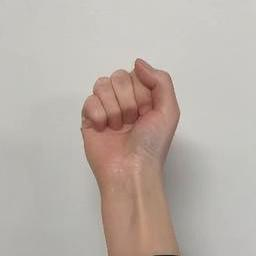} & 
    \includegraphics[width=0.13\textwidth]{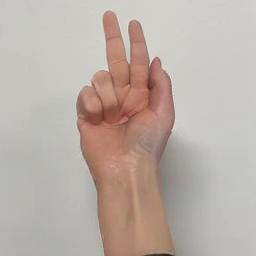} & 
    \includegraphics[width=0.13\textwidth]{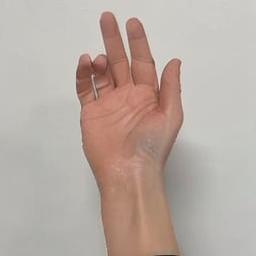} & 
    \includegraphics[width=0.13\textwidth]{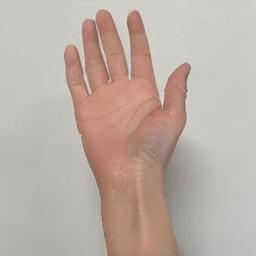} & 
    \includegraphics[width=0.13\textwidth]{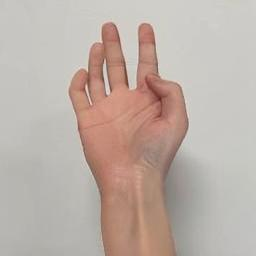} &
    \includegraphics[width=0.13\textwidth]{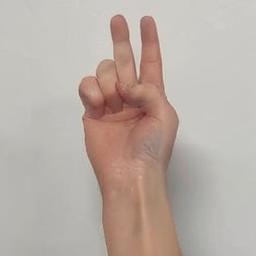} &
    \includegraphics[width=0.13\textwidth]{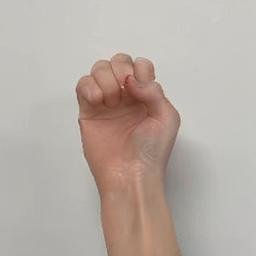} \\
    \rotatebox{90}{\hspace{1.0cm}\footnotesize GT\;}&
    &
    \includegraphics[width=0.13\textwidth]{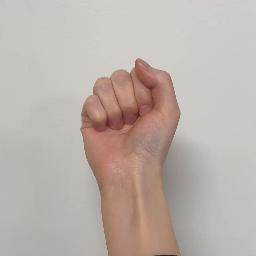} &
    \includegraphics[width=0.13\textwidth]{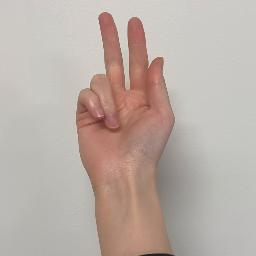} &
    \includegraphics[width=0.13\textwidth]{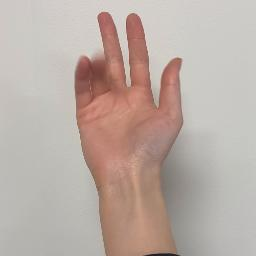} &
    \includegraphics[width=0.13\textwidth]{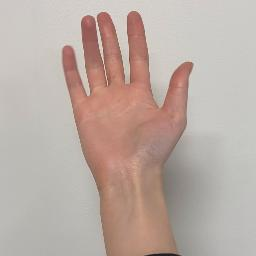} &
    \includegraphics[width=0.13\textwidth]{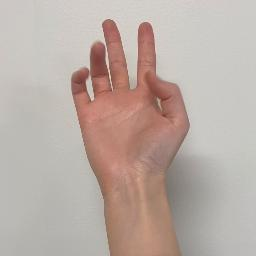} &
    \includegraphics[width=0.13\textwidth]{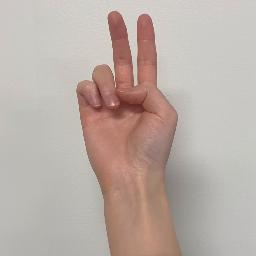} &
    \includegraphics[width=0.13\textwidth]{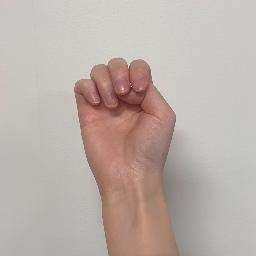} &\\[3.0pt]
    \rotatebox{90}{\hspace{1.0cm} \footnotesize\cite{controlnext}} & 
    \; &
    \includegraphics[width=0.13\textwidth]{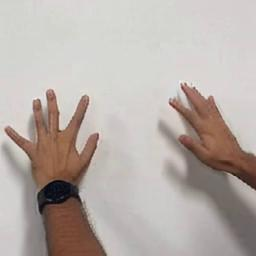} & 
    \includegraphics[width=0.13\textwidth]{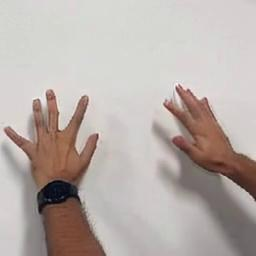} & 
    \includegraphics[width=0.13\textwidth]{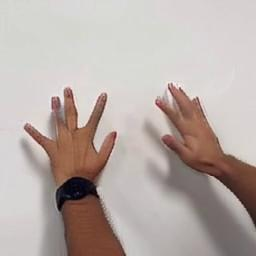} & 
    \includegraphics[width=0.13\textwidth]{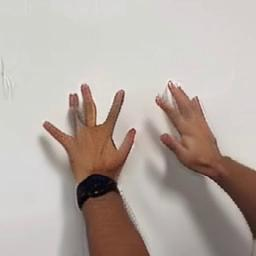} & 
    \includegraphics[width=0.13\textwidth]{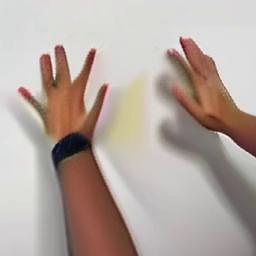} &
    \includegraphics[width=0.13\textwidth]{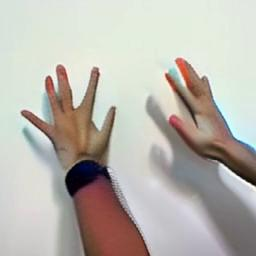} &
    \includegraphics[width=0.13\textwidth]{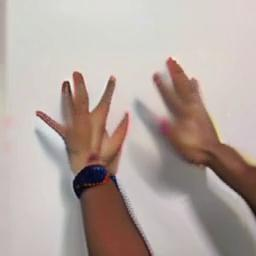} \\
    \rotatebox{90}{\hspace{1.0cm}\footnotesize \cite{animate_anyone}\;}&
    &
    \includegraphics[width=0.13\textwidth]{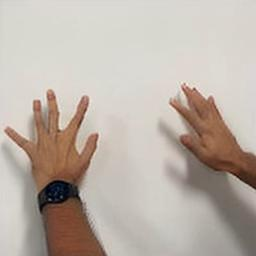} & 
    \includegraphics[width=0.13\textwidth]{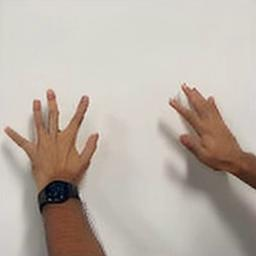} & 
    \includegraphics[width=0.13\textwidth]{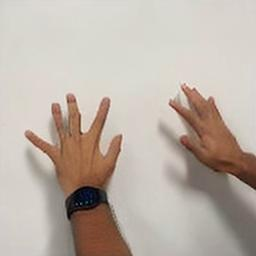} & 
    \includegraphics[width=0.13\textwidth]{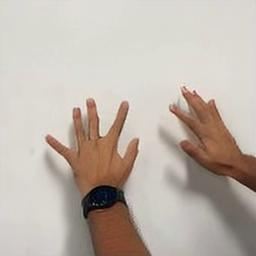} & 
    \includegraphics[width=0.13\textwidth]{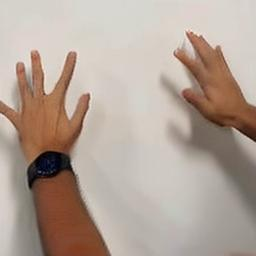} &
    \includegraphics[width=0.13\textwidth]{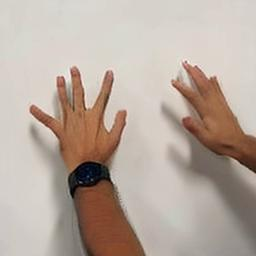} &
    \includegraphics[width=0.13\textwidth]{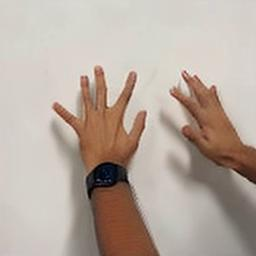} \\
    \rotatebox{90}{\hspace{1.0cm}\footnotesize Ours\;}&
    &
    \includegraphics[width=0.13\textwidth]{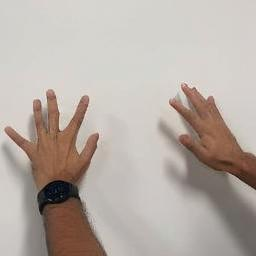} & 
    \includegraphics[width=0.13\textwidth]{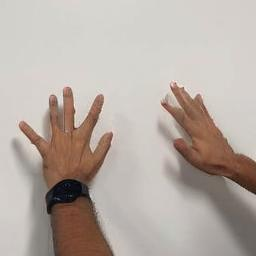} & 
    \includegraphics[width=0.13\textwidth]{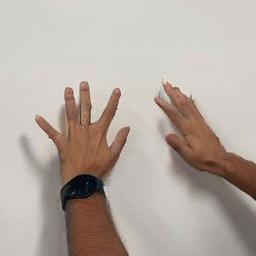} & 
    \includegraphics[width=0.13\textwidth]{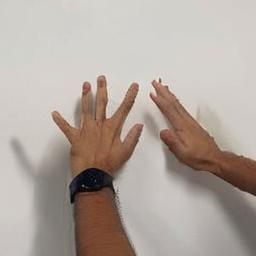} & 
    \includegraphics[width=0.13\textwidth]{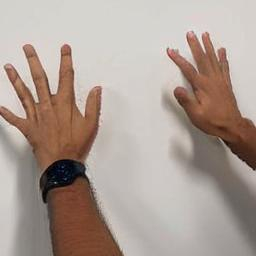} &
    \includegraphics[width=0.13\textwidth]{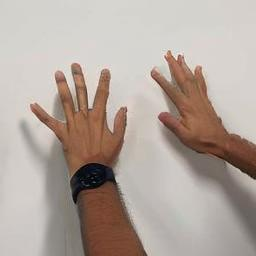} &
    \includegraphics[width=0.13\textwidth]{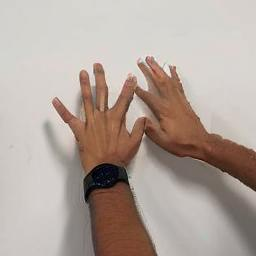} \\
    \rotatebox{90}{\hspace{1.0cm}\footnotesize GT\;}&
    &
    \includegraphics[width=0.13\textwidth]{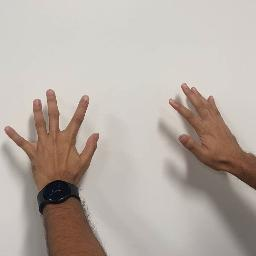} &
    \includegraphics[width=0.13\textwidth]{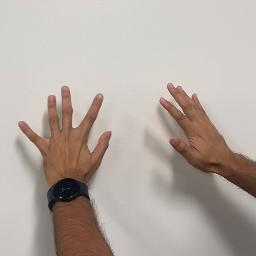} &
    \includegraphics[width=0.13\textwidth]{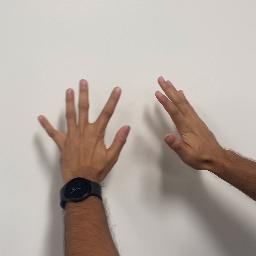} &
    \includegraphics[width=0.13\textwidth]{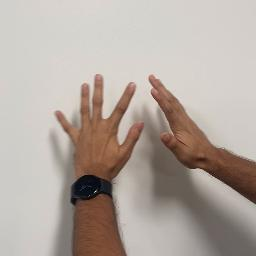} &
    \includegraphics[width=0.13\textwidth]{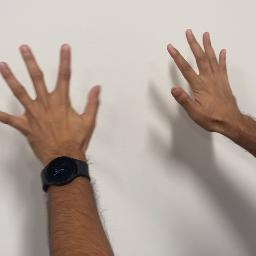} &
    \includegraphics[width=0.13\textwidth]{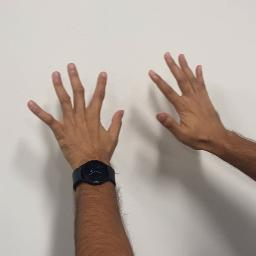} &
    \includegraphics[width=0.13\textwidth]{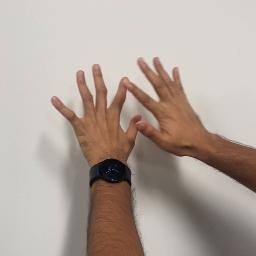} &\\[4.0pt]
    && Reference& \multicolumn{6}{c}{Time} \vspace{.5em}\\
    &&& \multicolumn{6}{c}{
        \begin{tikzpicture}
            \draw[->, line width=0.3mm] (0,0) -- (11.5,0);
        \end{tikzpicture}} \\
    \end{tabular}
    \caption{Given the first frame image and a sequence of 2D keypoints captured in the wild by an iphone camera, \modelname can autoregressively generate a motion-controlled video, despite not explicitly trained on videos. This shows our model's high versatility and potentials for being used in various applications. ControlNeXt~\cite{controlnext} and AnimateAnyone~\cite{animate_anyone} struggles to follow the pose change or present significant visual artifacts while our model demonstrate robust generalization and emergent understanding of some physical effects such as casted shadows.}
    \label{fig:suppl_video}
\end{figure*}
